# Supplementary material for: Search for squarks and gluinos in events with isolated leptons, jets and missing transverse momentum at $\sqrt{s}=8$ TeV with the ATLAS detector
Source: arXiv:1501.03555 source file (2015-05-04)
Supplement: Supplementary file 1 [file appendix.tex]

\clearpage
\appendix
\section{Auxiliary material}

\subsection{Additional information}
\subsubsection{Additional plots for the control regions}

\begin{figure}[htb]
\centering
\includegraphics[width=0.3\textwidth]{figures/can_h1L_TR3J_noupmtEM_mt_afterFit.eps}
\includegraphics[width=0.3\textwidth]{figures/can_h1L_TR5J_noupmtEM_mt_afterFit.eps}
\includegraphics[width=0.3\textwidth]{figures/can_h1L_TR6J_noupmtEM_mt_afterFit.eps}
\includegraphics[width=0.3\textwidth]{figures/can_h1L_WR3J_noupmtEM_mt_afterFit.eps}
\includegraphics[width=0.3\textwidth]{figures/can_h1L_WR5J_noupmtEM_mt_afterFit.eps}
\includegraphics[width=0.3\textwidth]{figures/can_h1L_WR6J_noupmtEM_mt_afterFit.eps}
\caption{\mt~distribution, prior to the upper \mt~cut, in the 3-jet (left), 5-jet (middle) and 6-jet (right) \ttbar~(top) and
$W$+jets (bottom) control regions used in the hard single-lepton channels.
The ``Data/SM'' plots show the ratio of data to the summed Standard Model expectation.
The Standard Model expectation is derived from the fit described in section \ref{sec:bkgfit}. The uncertainty band on the Standard Model expectation shown here
combines the statistical uncertainty on the simulated event samples with the systematic uncertainties.
The last bin includes the overflow. For illustration, the expected signal
distributions are shown for gluino pair production with
 with $m_{\tilde{g}}=1025 \GeV, m_{\tilde{\chi}^{\pm}_{1}}=545 \GeV$ and $m_{\tilde{\chi}^0_1}=65 \GeV$.
} \label{fig:1hardCR_MT}
\end{figure}

\begin{figure}[htb]
\centering
\includegraphics[width=0.3\textwidth]{../INT/SoftLepton/figures/Appendix/ISR_SRCR_PAPER/met_3J_CRnometUP_T_Comb.eps}
\includegraphics[width=0.3\textwidth]{../INT/SoftLepton/figures/Appendix/ISR_SRCR_PAPER/met_5J_CRnometUP_T_Comb.eps}
\includegraphics[width=0.3\textwidth]{../INT/SoftLepton/figures/Appendix/ISR_SRCR_PAPER/met_new3J_CRnometUP_T_Comb.eps}
\includegraphics[width=0.3\textwidth]{../INT/SoftLepton/figures/Appendix/ISR_SRCR_PAPER/met_3J_CRnometUP_W_Comb.eps}
\includegraphics[width=0.3\textwidth]{../INT/SoftLepton/figures/Appendix/ISR_SRCR_PAPER/met_5J_CRnometUP_W_Comb.eps}
\includegraphics[width=0.3\textwidth]{../INT/SoftLepton/figures/Appendix/ISR_SRCR_PAPER/met_new3J_CRnometUP_W_Comb.eps}

\caption{\met~distribution, before the upper \met~cut is applied, in the 3-jet (left), 5-jet (middle) and 3-jet inclusive (right) \ttbar~(top) and $W$+jets (bottom) control 
regions used in the soft single-lepton channels.
The ``Data/SM'' plots show the ratio of data to the summed Standard Model expectation.
The Standard Model expectation is derived from the fit described in section \ref{sec:bkgfit}. The uncertainty band on the Standard Model expectation shown here
combines the statistical uncertainty on the simulated event samples with the systematic uncertainties.
The last bin includes the overflow.
For illustration, the expected signal distribution is shown
for first- and second-generation squark pair production with $m_{\tilde{q}}=425$ \GeV, $m_{\tilde{\chi}^{\pm}_{1}}$=385 \GeV~and $m_{\tilde{\chi}^0_1}=345$ \GeV,
$m_{\tilde{q}}=300$ \GeV, $m_{\tilde{\chi}^{\pm}_{1}}$=110 \GeV~and $m_{\tilde{\chi}^0_1}=60$ \GeV, and for gluino pair production with
$m_{\tilde{g}}=625$ \GeV, $m_{\tilde{\chi}^{\pm}_{1}}$=545 \GeV~and
$m_{\tilde{\chi}^0_1}=465$ \GeV.
} \label{fig:1softCR_MET}
\end{figure}

\begin{figure}[ht]
\centering
\includegraphics[width=0.45\textwidth]{figures/stacks2L/AppendixCR/can_Z_CRSF_LM_MR_afterFit.eps}
\includegraphics[width=0.45\textwidth]{figures/stacks2L/AppendixCR/can_Z_CRSF_HM_MR_afterFit.eps}
\includegraphics[width=0.45\textwidth]{figures/stacks2L/AppendixCR/can_T_CRSF_LM_MR_afterFit.eps}
\includegraphics[width=0.45\textwidth]{figures/stacks2L/AppendixCR/can_T_CRSF_HM_MR_afterFit.eps}
\includegraphics[width=0.45\textwidth]{figures/stacks2L/AppendixCR/can_T_CREM_LM_MR_afterFit.eps}
\includegraphics[width=0.45\textwidth]{figures/stacks2L/AppendixCR/can_T_CREM_HM_MR_afterFit.eps}
\caption{$M_R'$~distribution in the low-multiplicity (left) and 3-jet (right) $Z$ (top) control region and in the \ttbar~ control region with same-flavour (middle)
or opposite-flavour (bottom) leptons used in the hard dilepton channels.
The ``Data/SM'' plots show the ratio of data to the summed Standard Model expectation.
The Standard Model expectation is derived from the fit described in section \ref{sec:bkgfit}. The uncertainty band on the Standard Model expectation shown here
combines the statistical uncertainty on the simulated event samples with the systematic uncertainties. For illustration, the expected signal
distributions are shown for squark pair production with $m_{\tilde{q}}=825 \GeV, m_{\tilde{\chi}^{\pm}_{1}/\tilde{\chi}^{0}_{2}}=465 \GeV, m_{\tilde{\ell}/\tilde{\nu}}=285 \GeV$ and $m_{\tilde{\chi}^0_1}=105 \GeV$.
} \label{fig:2hardCR2b}
\end{figure}

\clearpage
\subsubsection{Event yields and plots in the other hard dilepton signal regions}

  \begin{figure}[htb]
  \centering
   \includegraphics[width=0.49\textwidth]{figures/stacks2L/Appendix2LSR/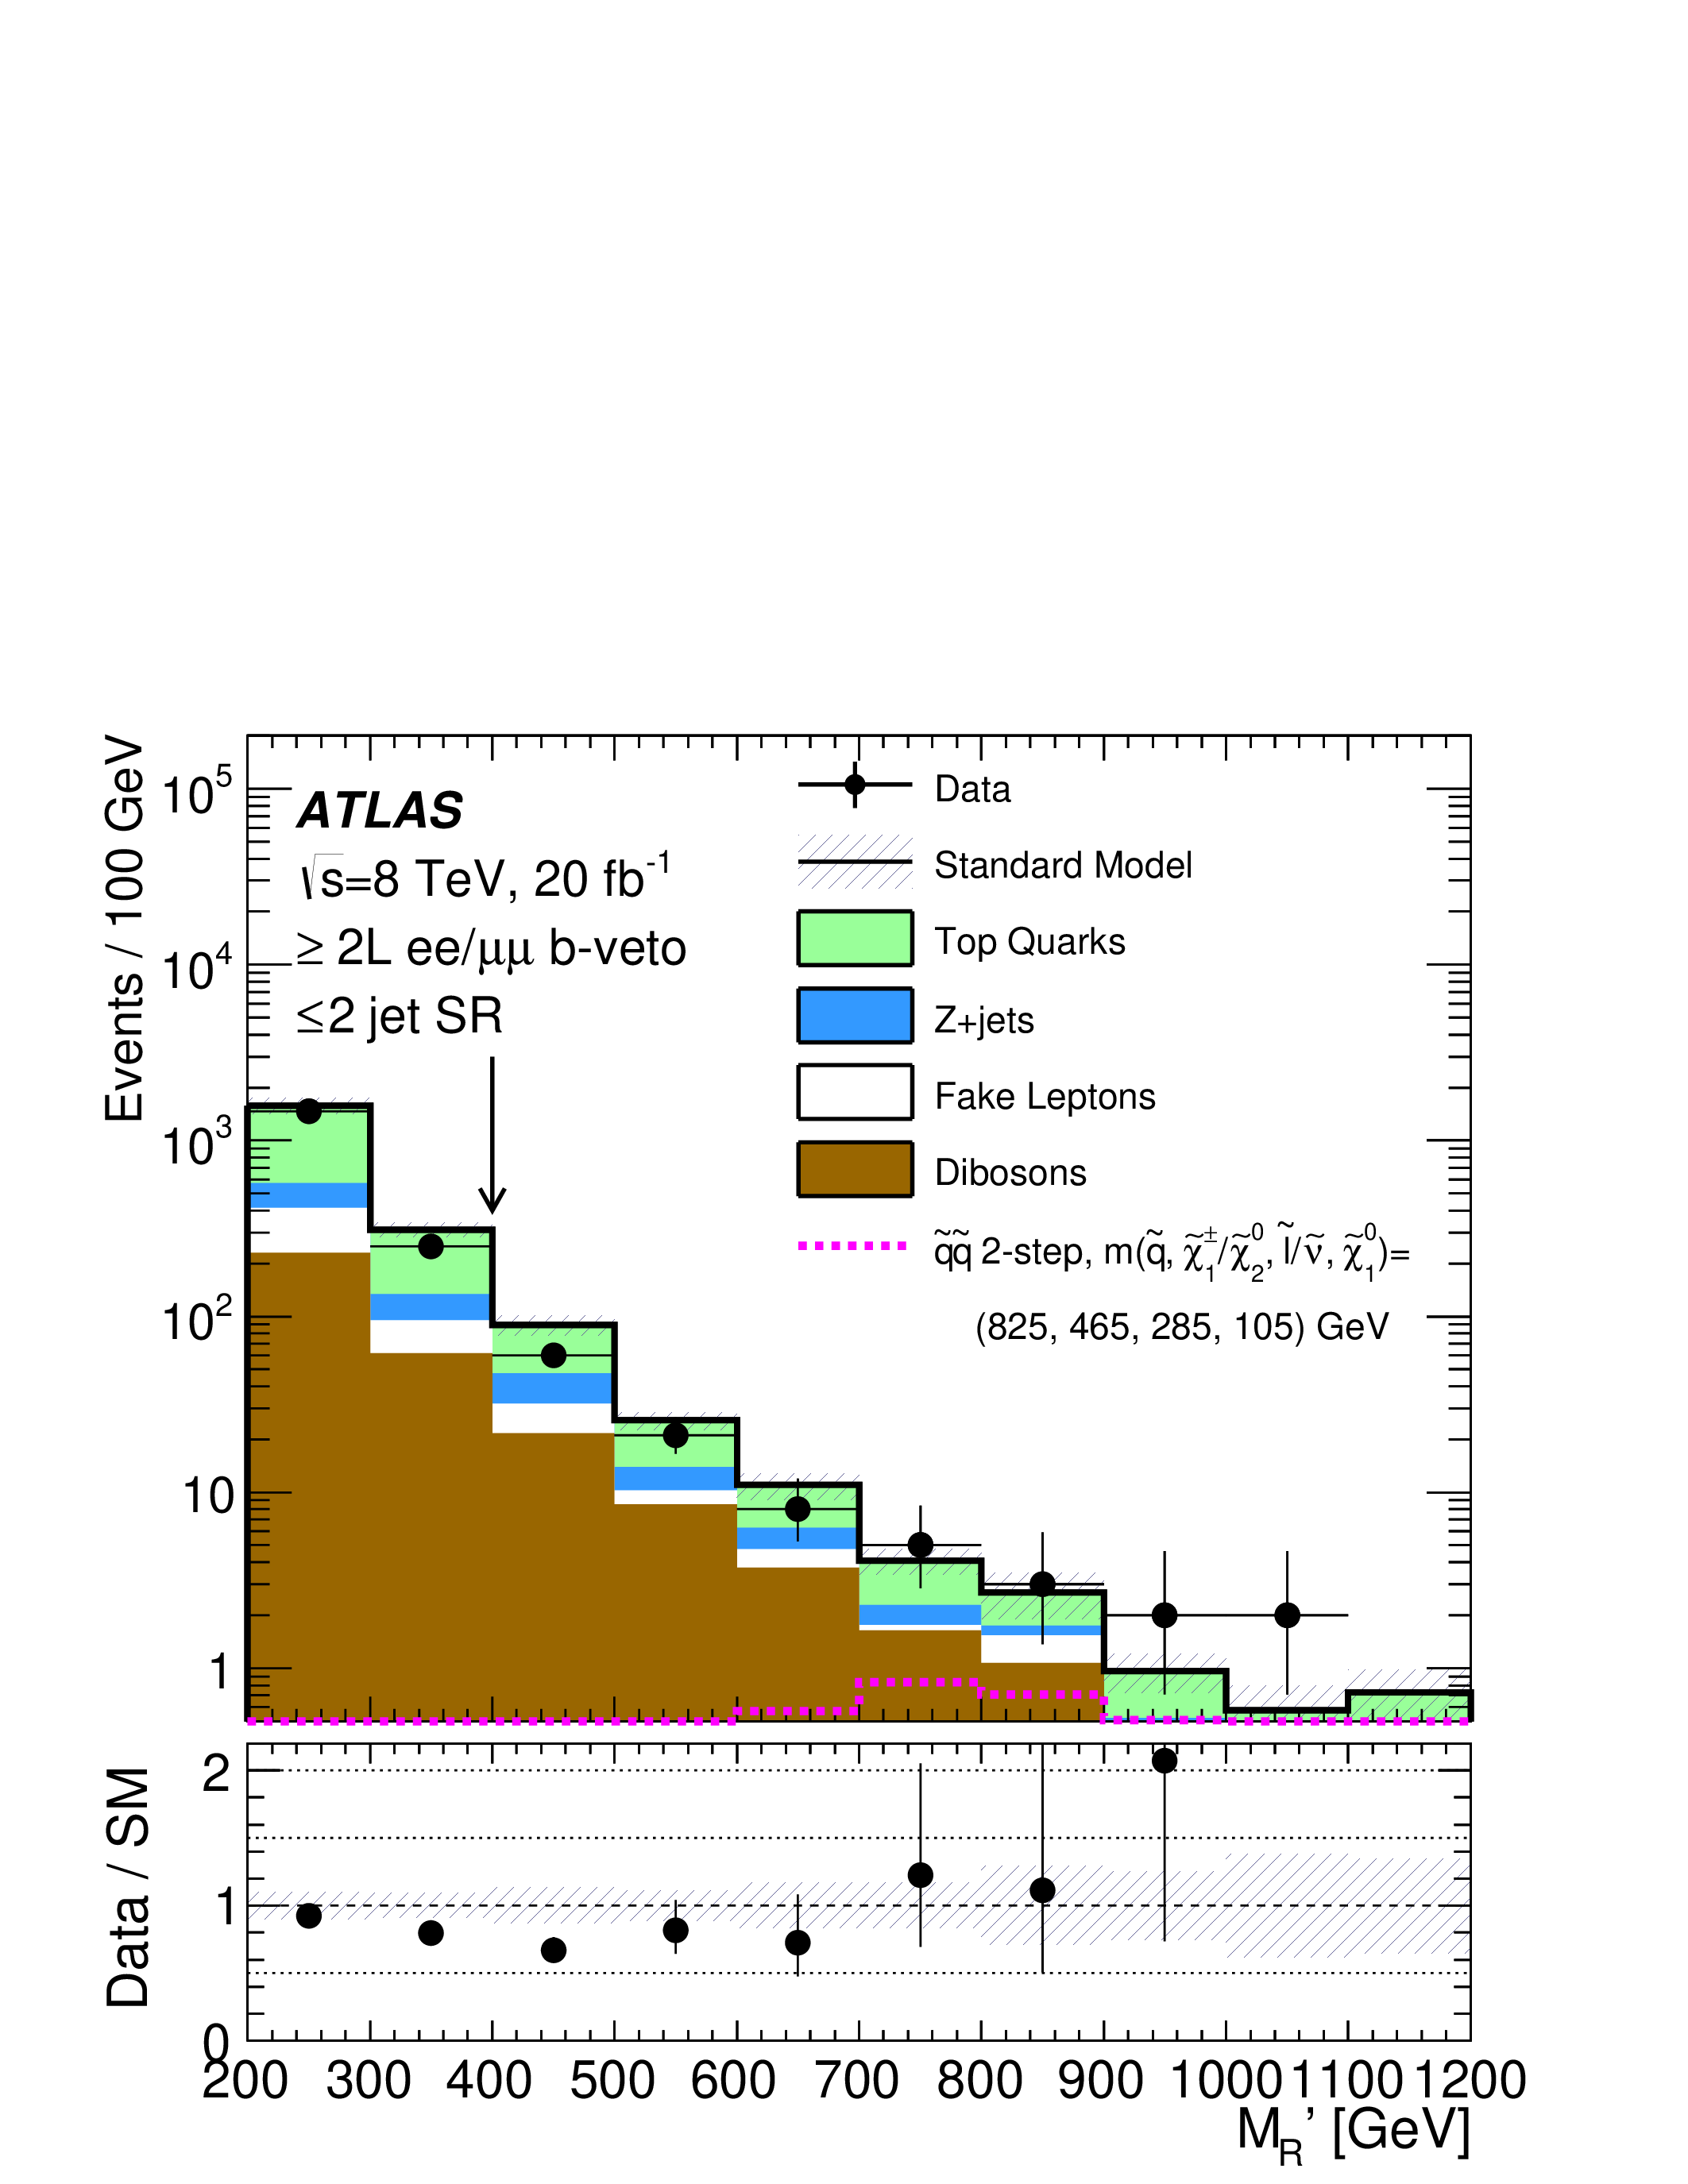}
   \includegraphics[width=0.49\textwidth]{figures/stacks2L/Appendix2LSR/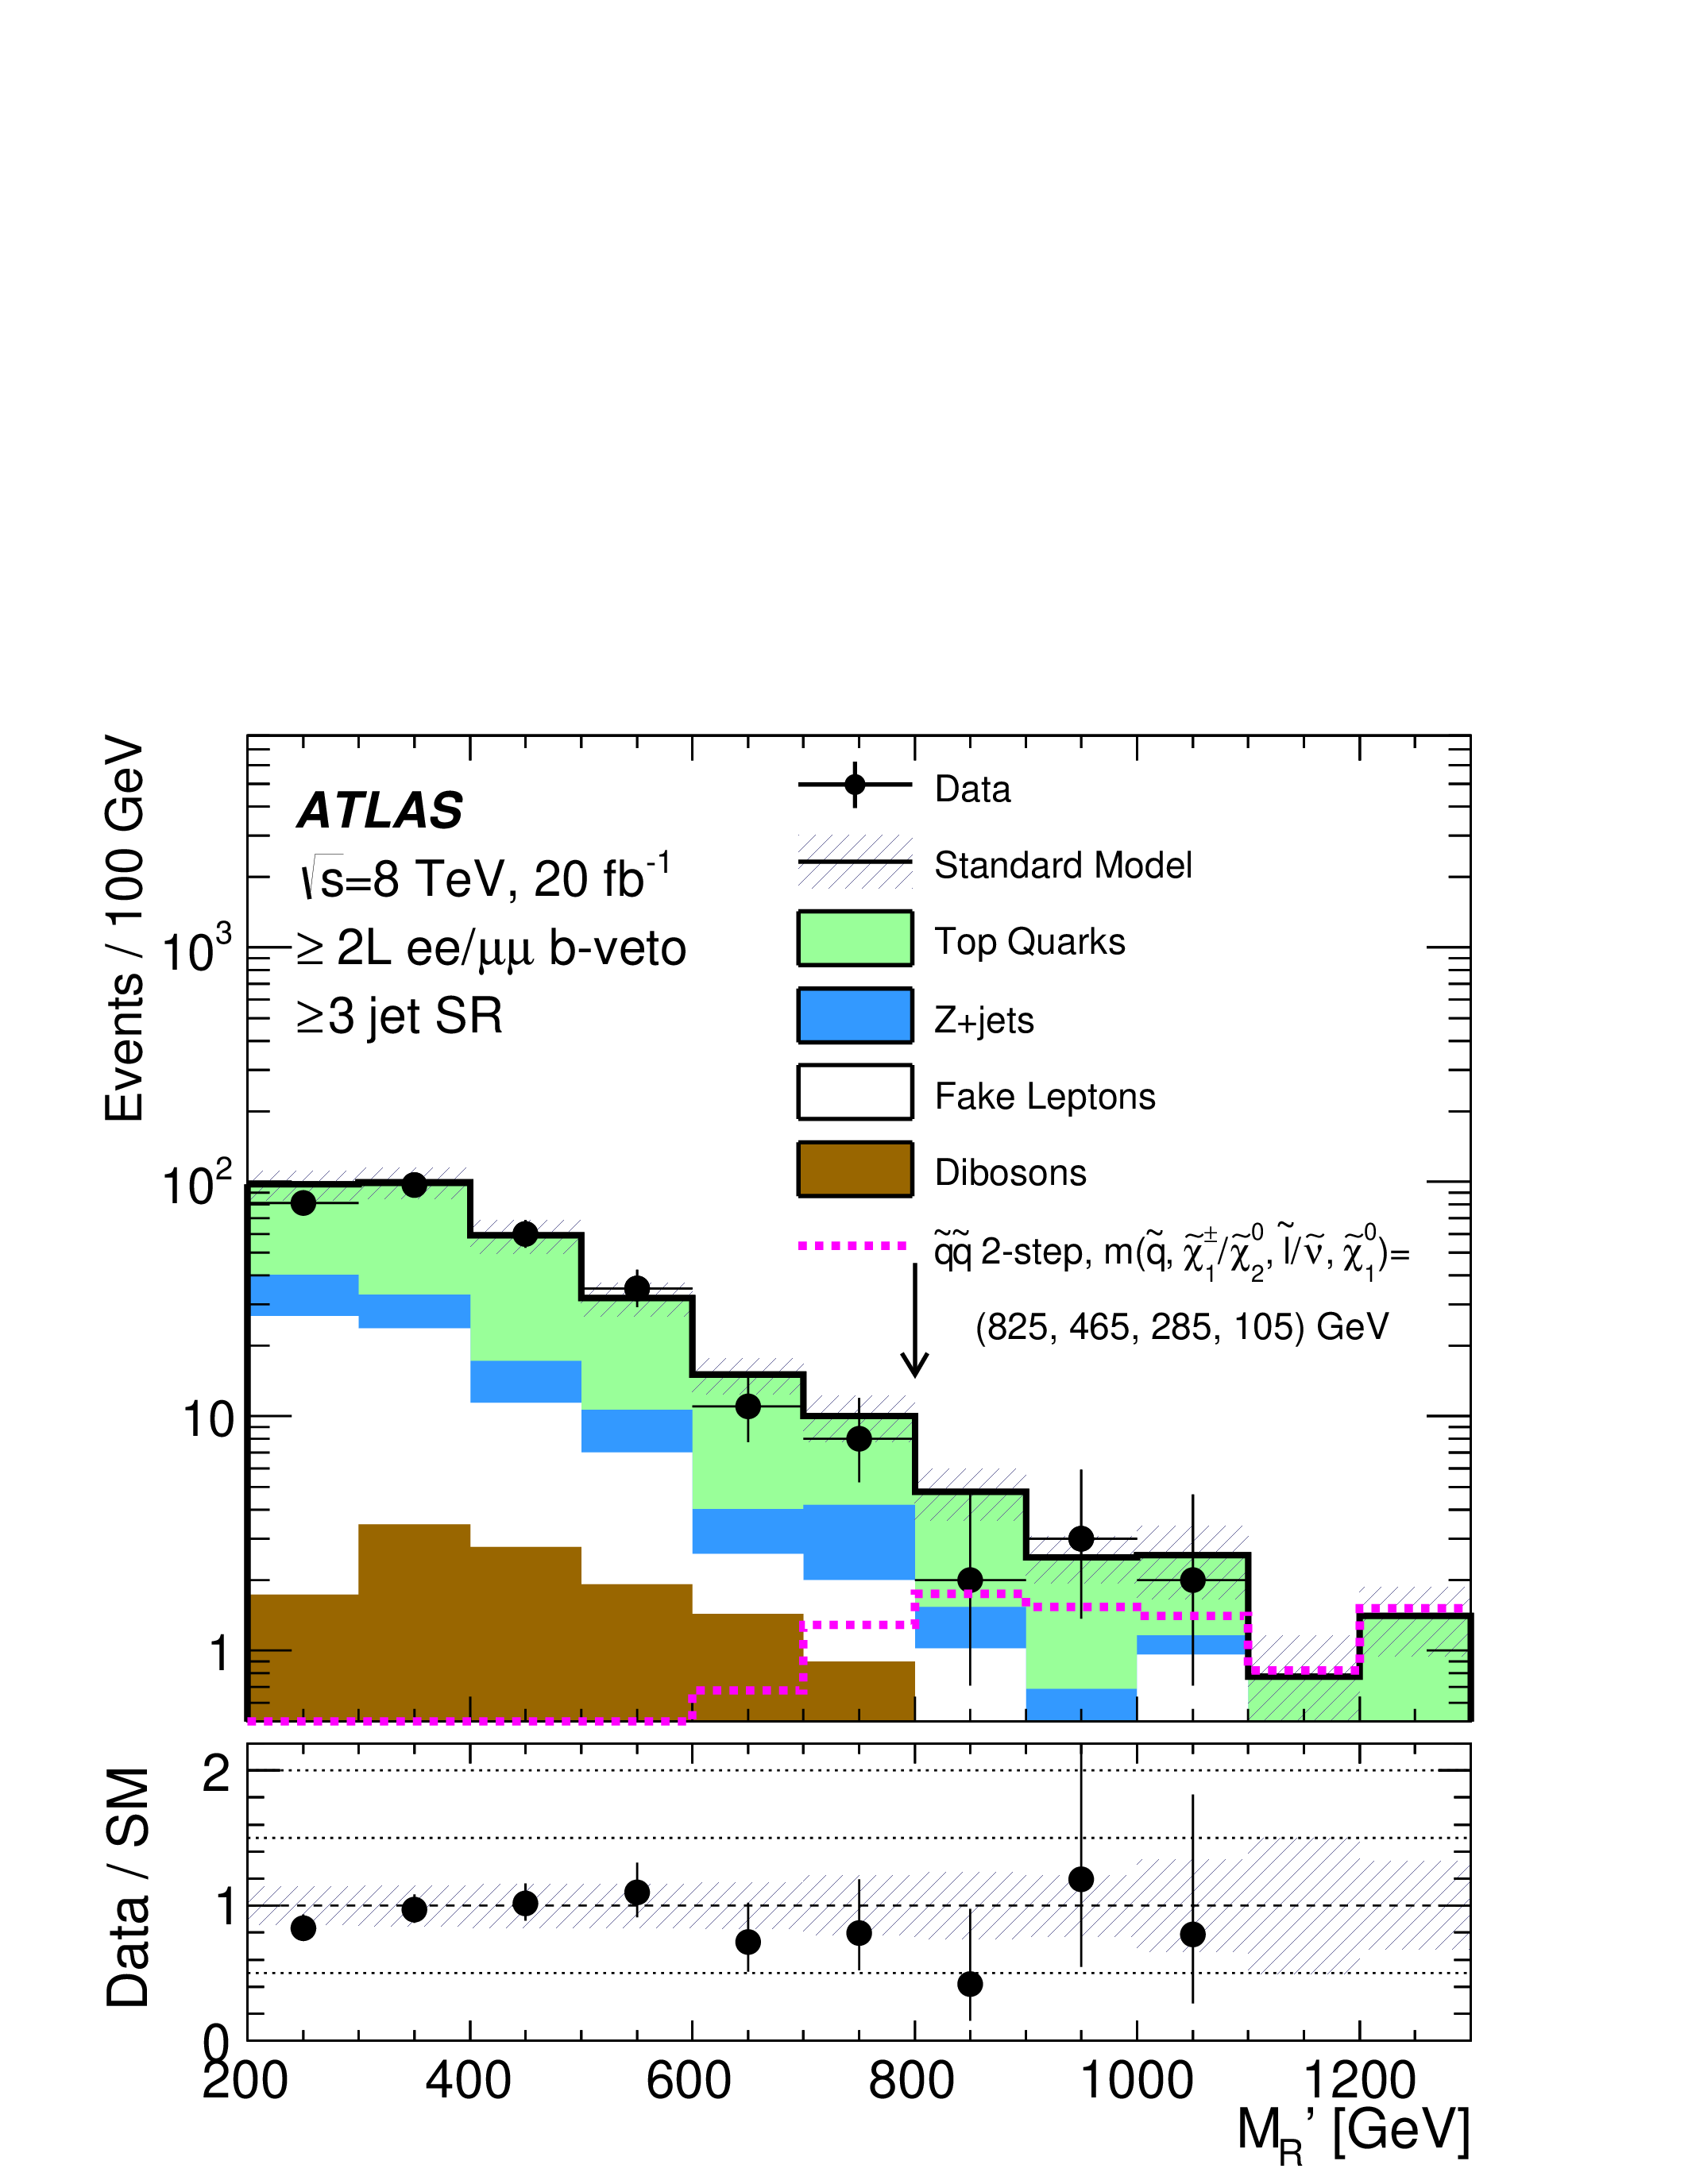}
   \includegraphics[width=0.49\textwidth]{figures/stacks2L/Appendix2LSR/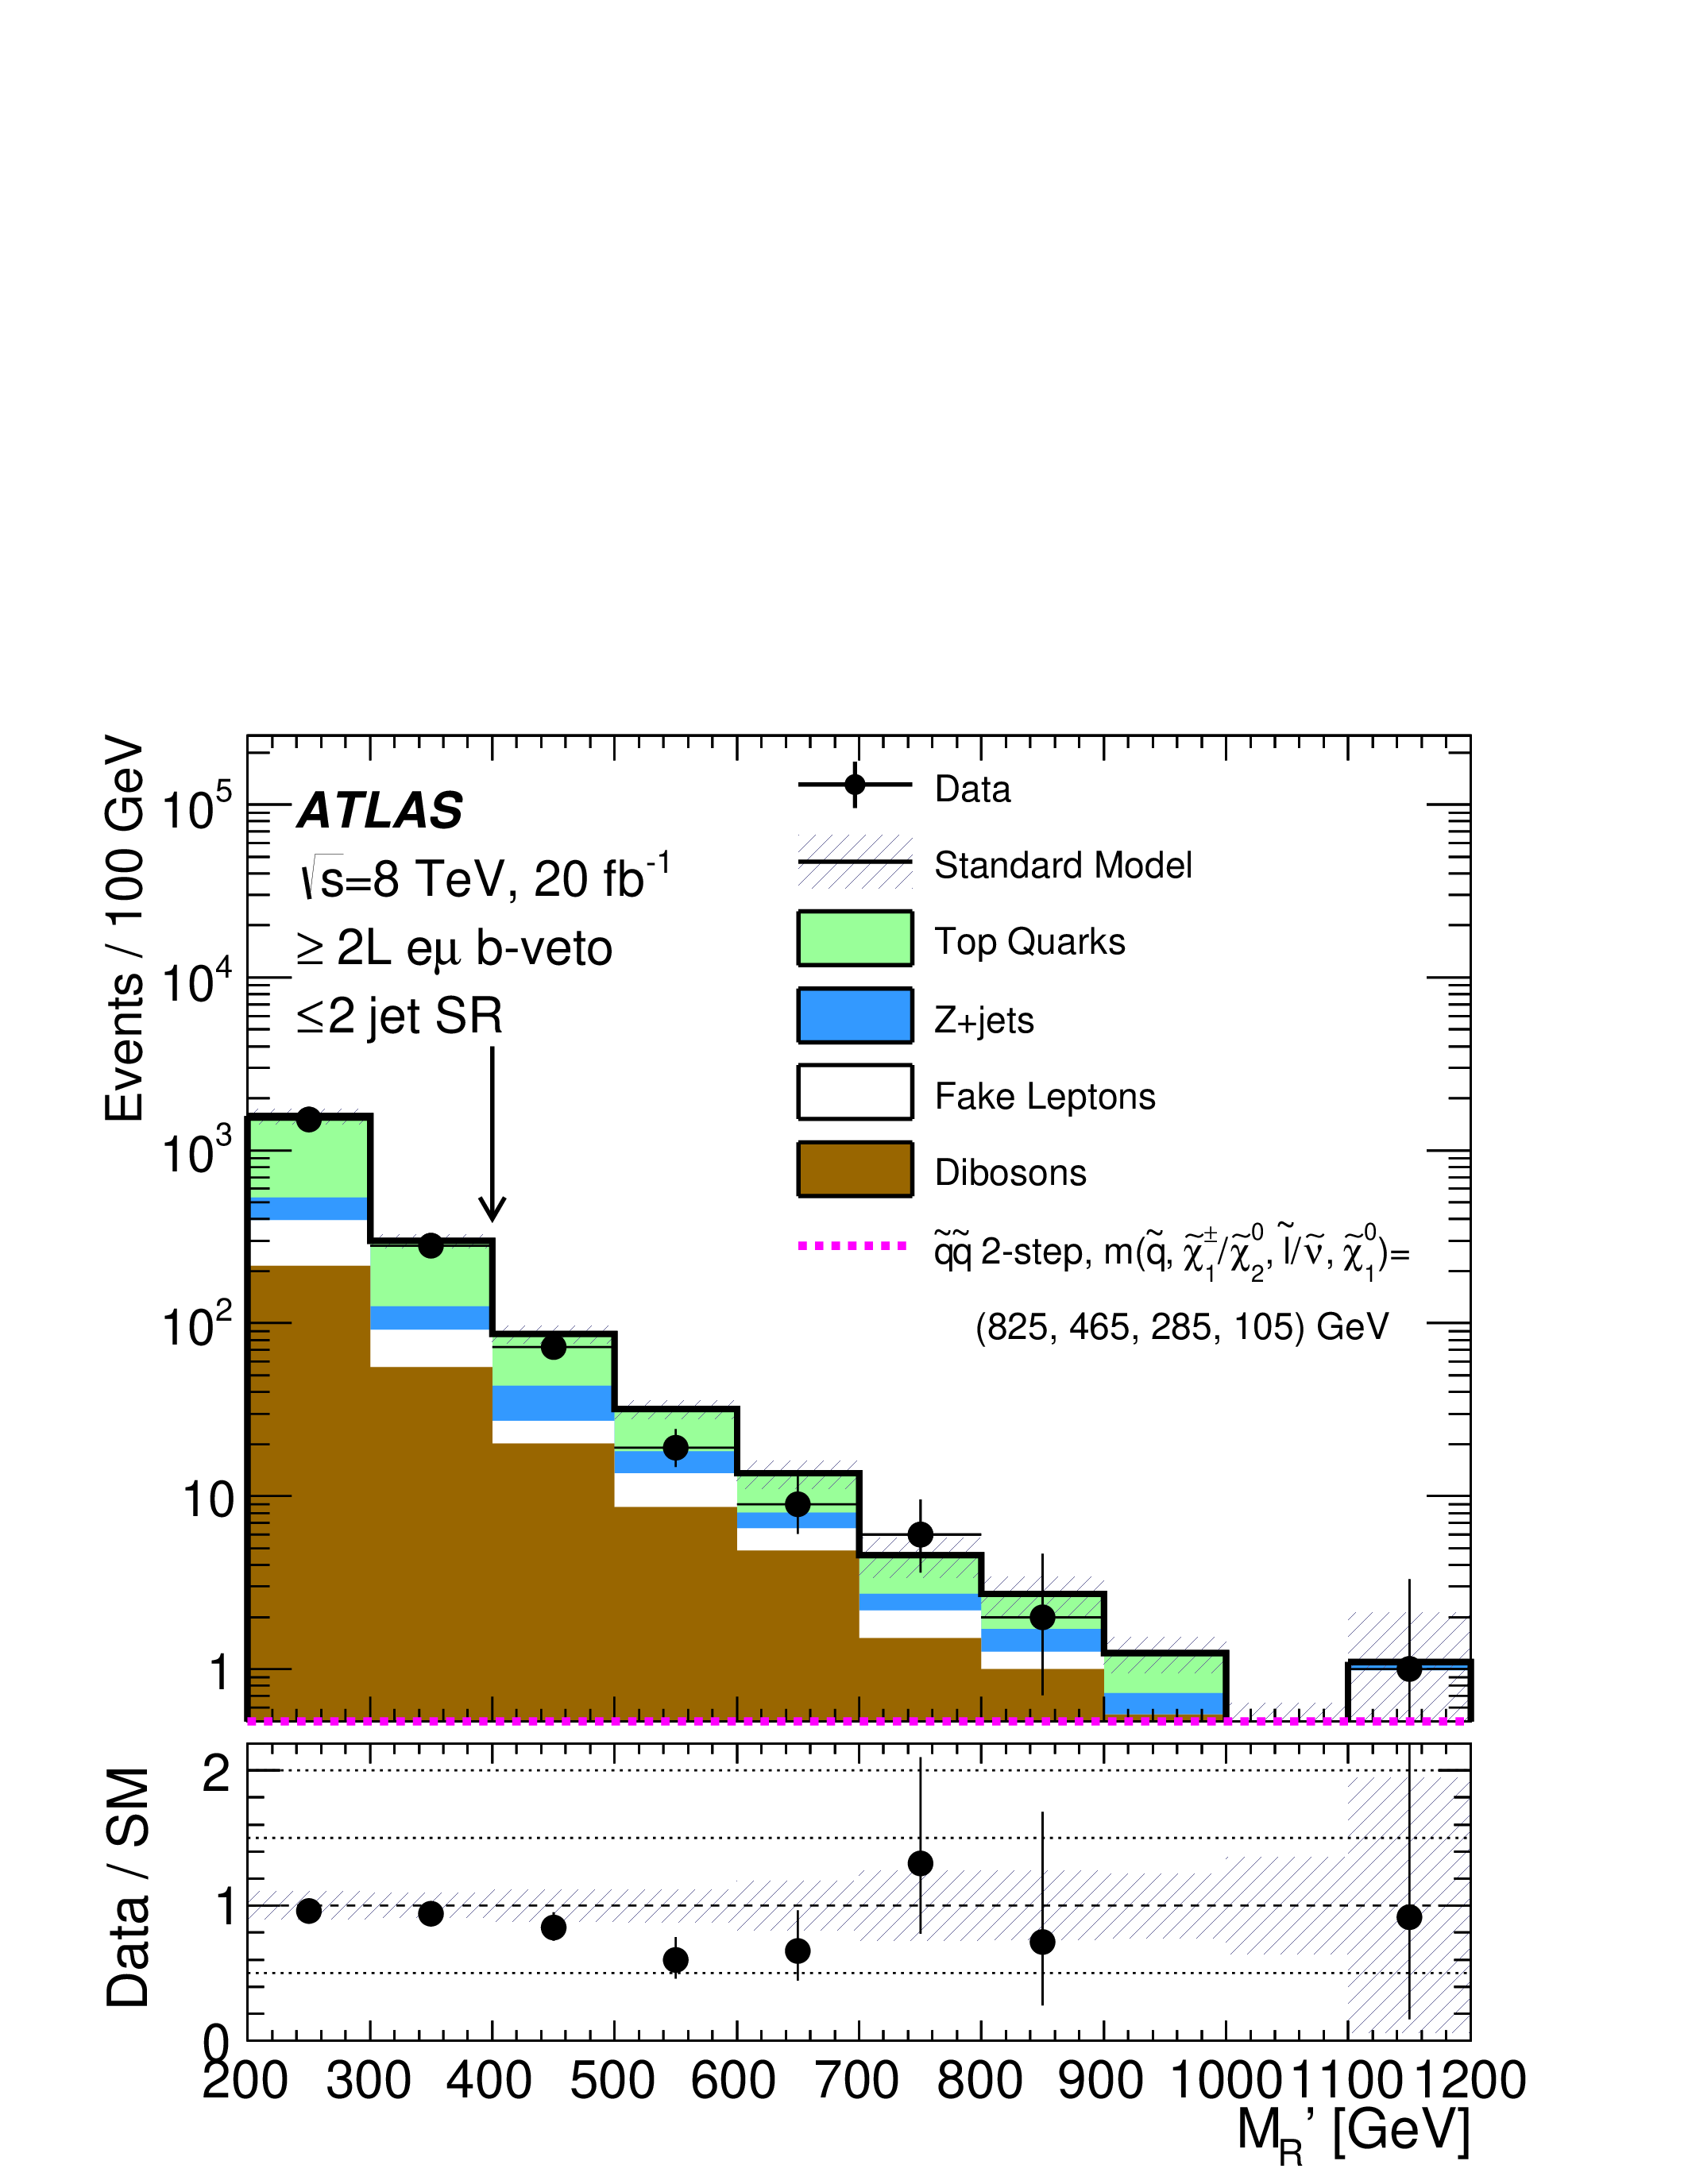}
   \includegraphics[width=0.49\textwidth]{figures/stacks2L/Appendix2LSR/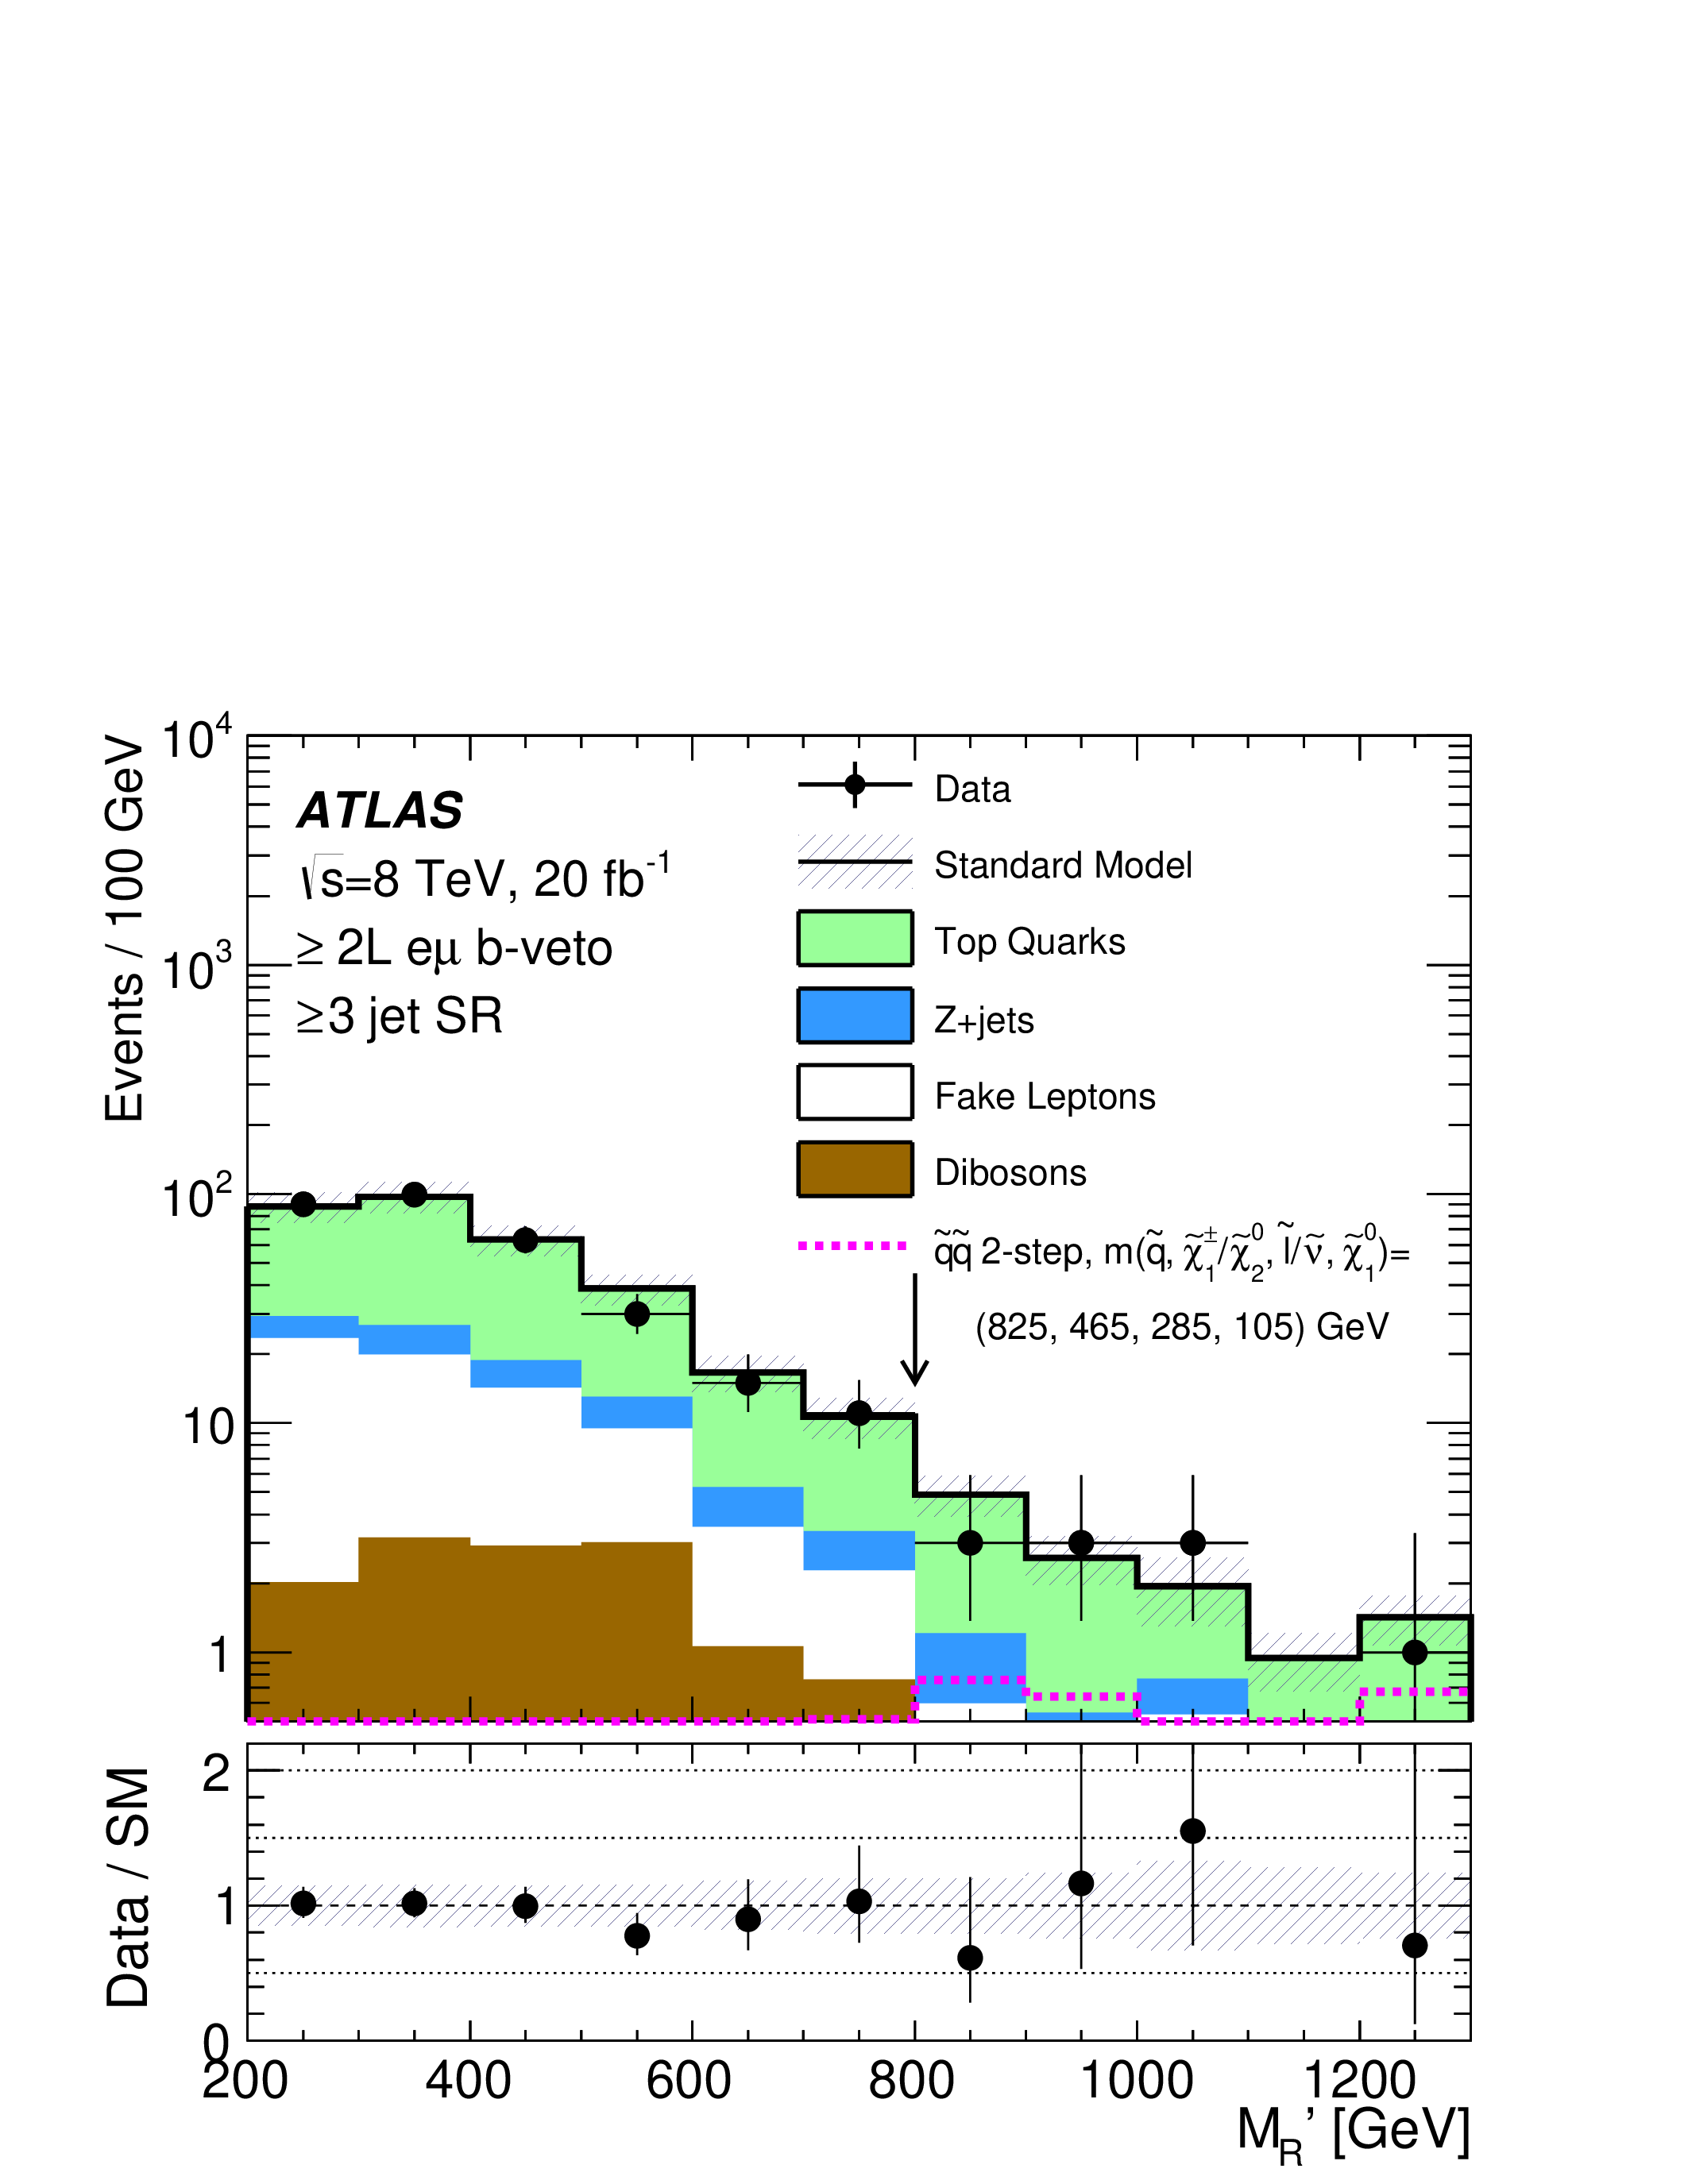}
   \caption{The distribution in $M_R'$, after the background fit, in the same-flavour (top) and opposite-flavour (bottom) hard dilepton channels for the
low-multiplicity (left) and 3-jet (right) signal regions requesting exactly two leptons. Statistical and systematic uncertainties are indicated. For illustration, the expected signal
distributions are shown for squark pair production with $m_{\tilde{q}}=825 \GeV, m_{\tilde{\chi}^{\pm}_{1}/\tilde{\chi}^{0}_{2}}=465 \GeV, m_{\tilde{\ell}/\tilde{\nu}}=285 \GeV$ and $m_{\tilde{\chi}^0_1}=105 \GeV$.
}
   \label{fig:2LSR_MR}
 \end{figure}

  \begin{figure}[htb]
  \centering
   \includegraphics[width=0.49\textwidth]{figures/stacks2L/Appendix2LOSSR/can_VSR_SF_LM_MR_afterFit.eps}
   \includegraphics[width=0.49\textwidth]{figures/stacks2L/Appendix2LOSSR/can_VSR_SF_HM_MR_afterFit.eps}
   \includegraphics[width=0.49\textwidth]{figures/stacks2L/Appendix2LOSSR/can_VSR_EM_LM_MR_afterFit.eps}
   \includegraphics[width=0.49\textwidth]{figures/stacks2L/Appendix2LOSSR/can_VSR_EM_HM_MR_afterFit.eps}
   \caption{The distribution in $M_R'$, after the background fit, in the same-flavour (top) and opposite-flavour (bottom) hard dilepton channels
for the low-multiplicity (left) and 3-jet (right) signal regions requesting two leptons of opposite sign. Statistical and systematic uncertainties are indicated. For illustration, the expected signal
distributions are shown for squark pair production with $m_{\tilde{q}}=825 \GeV, m_{\tilde{\chi}^{\pm}_{1}/\tilde{\chi}^{0}_{2}}=465 \GeV, m_{\tilde{\ell}/\tilde{\nu}}=285 \GeV$ and $m_{\tilde{\chi}^0_1}=105 \GeV$.
}
   \label{fig:OS2LSR_MR}
 \end{figure}

\input{texfiles/2l_BG_2LSR.tex}
\input{texfiles/2l_BG_OS2LSR.tex}
\input{texfiles/2l_BG_DR.tex}

\clearpage
\subsection{Auxiliary material for HepData}
\subsubsection{Cut flow tables for benchmark signal models}
 
\begin{table}[hbt]
%\scriptsize
\tiny
\begin{center}
\begin{tabular}{|lccc|}
\hline
 & \gluino\gluino & \squark\squark & \squark\squark \\ 
Cut & $(m_{\gluino},m_{\chinoonepm},m_{\ninoone})=$ & $(m_{\squark},m_{\chinoonepm},m_{\ninoone}) =$ & $(m_{\squark},m_{\chinoonepm},m_{\ninoone})=$ \\
 & (625,545,465) \GeV & (425,385,345) \GeV & (300,110,60) \GeV \\
\hline
\multicolumn{4}{|c|}{ Common preselection } \\
\hline
No cuts                        &  19603.4 &   19250.2& 157946.9 \\
\met\ trigger requirement      &   8633.6 &    6859.4& 101747.8 \\
Reject events with bad jets    &   8595.5 &    6827.7& 101261.7 \\
Reject events with bad muons   &   8595.5 &    6827.2& 101261.7 \\
Primary vertex $\ge 4$ tracks  &   8595.4 &    6827.2& 101251.7 \\
Veto events with cosmic muons  &   8555.2 &    6810.5& 100919.1 \\
At least 1 lepton             &   3177.8 &    2011.5&  34867.7 \\
Fake $E_{\text{T}}^{miss}$     &   3141.4 &    1995.0&  34398.1 \\
Lepton isolation, \pt$<$25\GeV & $675.1 $&$1022.5 $&$ 11816.9 $\\ 
\met$>150$ \GeV~,~\pt$^{\mathrm{jet},1}>130$ \GeV & $226.1 $&$343.8 $&$ 4360.8 $\\
\hline\hline
\multicolumn{4}{|c|}{ soft single-lepton 3-jet signal region } \\
\hline
$3 \le N_{jet} < 5$ &  $23.4$&$79.4$& \\%$ 916.479 \pm 60.8596 $\\
$\mt > 100\,\GeV$ &$6.24$&$18.5 $&\\%$ 66.6169 \pm 15.8536 $\\
$\met> 400 \GeV$, $\met / \meff>0.3$ &$0 \pm 0$&$3.0^{+0.9\%}_{-1.2\%}$&\\ %$ 3.27812 \pm 3.27812 $\\ 
\hline
$\text{CL}_\text{S}$ obs (exp)  &  & 0.370 (0.405) & \\
\hline\hline
%Observed CLs & $-$ & 0.370 & \\\hline
%Expected CLs & $-$ & 0.405 & \\\hline
\multicolumn{4}{|c|}{ soft single-lepton 5-jet signal region } \\
\hline
$N_{jet} \geq 5$ &$120.2 $&$92.1$&\\%$ 844.015 \pm 58.8017 $\\
\mt $> 100$ \GeV & $55.8$&$28.1$& \\%$88.8558 \pm 19.1778 $\\
$\met> 300 \GeV$, $\met / \meff>0.3$  &  $19.1^{+6.0\%}_{-6.6\%}$  &$12.0^{+4.2\%}_{-2.5\%}$& \\%$ 11.1497 \pm 6.33964 $\\
\hline
$\text{CL}_\text{S}$ obs (exp)  & 0.016 (0.048) & 0.031 (0.085) & \\
\hline\hline
%Observed CLs & 0.016 & 0.031 & \\\hline
%Expected CLs & 0.048 & 0.085 & \\\hline
\multicolumn{4}{|c|}{ soft single-lepton 3-jet inclusive signal region } \\
\hline
$N_{jet} \geq 3$ %&$79.19 \pm 10.86$&$92.10 \pm 6.85$
&&&$ 2104.4 $\\
\mt $> 120$ \GeV %&$17.70 \pm 5.53$&$18.43 \pm 3.12$
&&&$ 63.8  $\\
$\met> 180 \GeV$, $N_{bjet} == 0$  %&$14.53 \pm 5.05$&$15.43 \pm 2.84$&
&&&$40.2^{+19.4\%}_{-14.4\%}$ \\
\hline
$\text{CL}_\text{S}$ obs (exp)  &  &  & 0.042 (0.058)\\\hline
%Observed CLs & & & 0.042 \\\hline
%Expected CLs & & & 0.058 \\\hline
\end{tabular}
\caption{Cutflow table for the soft single-lepton signal regions with representative target signal models. All samples are normalised to 20.1~\ifb, and the number of generated events is 20000 for the gluino signal model, and 60000 for both squark signal models. The total experimental systematic uncertainty on the signal yield is indicated at the last cut defining each signal region, along with the corresponding observed and expected $\text{CL}_\text{S}$ values.
%The statistical and systematic uncertainties on the signal yields are indicated for each signal region, 
%as are the observed and expected $CL_{s}$.}
}
\label{tab:cutflow_1L3J5J}
\end{center}
\end{table}

%%%%%%%%%%%%%%%%%%%%%%%%%  soft 1 lepton: raw number cutflow %%%%%%%%%%%%%%%%%%%%%%%%%%%%%%%%%%%%%%%%%%%%

\begin{table}[hbt]
%\scriptsize
\tiny
\begin{center}
\begin{tabular}{|lccc|}
\hline
 & \gluino\gluino & \squark\squark & \squark\squark \\ 
Cut & $(m_{\gluino},m_{\chinoonepm},m_{\ninoone})=$ & $(m_{\squark},m_{\chinoonepm},m_{\ninoone}) =$ & $(m_{\squark},m_{\chinoonepm},m_{\ninoone})=$ \\
 & (625,545,465) \GeV & (425,385,345) \GeV & (300,110,60) \GeV \\
\hline
\multicolumn{4}{|c|}{ Common preselection } \\
\hline
No cuts                        &  20000 &  60000 & 60000 \\
\met\ trigger requirement      &   8957 &  21535 & 38710 \\
Reject events with bad jets    &   8918 &  21419 & 38490 \\
Reject events with bad muons   &   8918 &  21418 & 38490 \\
Primary vertex $\ge 4$ tracks  &   8916 &  21418 & 38486 \\
Veto events with cosmic muons  &   8879 &  21347 & 38361 \\
At least 1 lepton             &   3229 &   6243 & 13276 \\
Fake $E_{\text{T}}^{miss}$     &   3189 &   6191 & 13106 \\
Lepton isolation, \pt$<$25\GeV & $698 $&$3156$&$ 4480 $\\ 
%\hline
\met$>150$\GeV~,~\pt$^{\mathrm{jet},1}>130$ \GeV & $220 $&$1035 $&$ 1680$\\
\hline\hline
\multicolumn{4}{|c|}{ soft single-lepton 3-jet signal region } \\
\hline
$3 \le N_{jet} < 5$ &  $21$&$224$& \\
$\mt > 100\,\GeV$ &$6$&$49 $&\\
$\met> 400 \GeV$, $\met / \meff>0.3$ &$0 $&$9$&\\
\hline
$\text{CL}_\text{S}$ obs (exp)  &  & 0.370 (0.405) & \\
\hline\hline
\multicolumn{4}{|c|}{ soft single-lepton 5-jet signal region } \\
\hline
$N_{jet} \geq 5$ &$118 $&$294$&\\
\mt $> 100$ \GeV & $54$&$81$& \\
$\met> 300 \GeV$, $\met / \meff>0.3$  &  $20$  &$40$& \\
\hline
$\text{CL}_\text{S}$ obs (exp)  & 0.016 (0.048) & 0.031 (0.085) & \\
\hline\hline
\multicolumn{4}{|c|}{ soft single-lepton 3-jet inclusive signal region } \\
\hline
$N_{jet} \geq 3$ 
&&&$ 804 $\\
\mt $> 120$ \GeV 
&&&$ 25  $\\
$\met> 180 \GeV$, $N_{bjet} == 0$  
&&&$ 17$ \\ 
\hline
$\text{CL}_\text{S}$ obs (exp)  &  &  & 0.042 (0.058)\\\hline
\end{tabular}
\caption{Cutflow table (raw number events) for the soft single-lepton signal regions with representative target signal models, along with the corresponding observed and expected $\text{CL}_\text{S}$ values.
}
\label{tab:cutflow_1L3J5Jraw}
\end{center}
\end{table}

\begin{table}[hbt]
\scriptsize
\begin{center}

\begin{tabular}{|l||cc|cc|}
\hline
& \multicolumn{4}{c|}{ Signal ($ R_{\mathrm{c}}^{-1}, \Lambda R_{\mathrm{c}} $) } \\
 Cut &\multicolumn{2}{c|}{(800,3)}&\multicolumn{2}{c|}{(800,10)}\\
&  $N_{\text{raw}}$  &  $N_{\text{weighted}}$  &  $N_{\text{raw}}$  &  $N_{\text{weighted}}$\\
\hline
No cuts                        &   20000 & 6848.4 &   20000 & 6082.5 \\
\met\ trigger requirement      &    6595 & 2226.5 &    9003 & 2747.5 \\
Reject events with bad jets    &    6567 & 2220.6 &    8969 & 2739.1 \\
Reject events with bad muons   &    6567 & 2220.6 &    8969 & 2739.1 \\
Primary vertex $\ge 4$ tracks  &    6567 & 2220.6 &    8966 & 2738.2 \\
Veto events with cosmic muons  &    6506 & 2201.3 &    8896 & 2718.3 \\
At least 2 leptons             &    2445 &  824.0 &    4232 & 1295.9 \\
Fake $E_{\text{T}}^{miss}$     &    2429 &  823.1 &    4195 & 1285.1 \\
\hline
OS $\mu$ & 675 & 239.8 & 1098 & 345.9\\
$\met>$180 GeV & 297 & 101.3 & 345 & 109.1\\
$N_{{\rm jets}} (p_{T}>25)\geq 2$  & 263 & 88.95 & 342 & 108.3\\
$p_{T,{\rm jet1}} >$ 80 GeV & 260 & 87.66 & 332 & 105.7\\
\hline
$M_{\mu\mu}>$15, $|M_{\mu\mu}-M_{Z}|>$10 & 141 & 48.23 & 287 & 90.96\\
$dR_{\text{min}}(\text{jet}, \mu_2)>1$ & 94 & 31.96 & 191 & 59.47\\
$p_{T}^{\mu 1}<$25 GeV & 94 & 31.96 & 116 & 33.74\\
b-veto & 77 & 24.41 & 90 & 25.83\\
\hline
$M_{\mu\mu}<$60 & 77 & 24.41 & 88 & 25.83\\
$m_T^{\mu 1}>$40 GeV & 56 & 19.66 & 68 & 20.77\\
%$\met / \meff>$0.3 & 54 & 19.62 & 63 & 20.19\\
$\met / \meff>$0.3 & 54 & $19.6^{+41.9\%}_{-33.6\%}$ & 63 & $20.2^{+12.6\%}_{-11.7\%}$\\
\hline
\hline
$\text{CL}_\text{S}$ obs (exp)  & \multicolumn{2}{c|}{ 0.004 (0.004)} & \multicolumn{2}{c|}{0.0002 (0.0002)} \\

\hline
\end{tabular}
\caption{Cutflow table for the soft dimuon channel for two representative mUED signal points. The signal samples are normalised to 20.1~\ifb, and the number of generated events divided by the generator efficiency is 154870 and 108266 for the ($R_{\mathrm{c}}^{-1}, \Lambda R_{\mathrm{c}}$) = (800,3) and (800,10) points respectively. The total experimental systematic uncertainty on the signal yield is indicated at the last cut defining each signal region, along with the corresponding observed and expected $\text{CL}_\text{S}$ values.
% The systematic and statistical uncertainties on the signal yield are shown in the signal region.  The last row shows the observed and the expected $\text{CL}_\text{S}$ values.}
}
\label{tab:cutflow_2MUrest}
 \end{center}
 \end{table}

\clearpage
\begin{table}
\scriptsize
\begin{center}
\setlength{\tabcolsep}{0.0pc}
\begin{tabular*}{\textwidth}{@{\extracolsep{\fill}}lcccc}
\noalign{\smallskip}\hline\noalign{\smallskip}
Cut     & & & &\\
     & \multicolumn{2}{c}{$N_\mathrm{raw}$} & \multicolumn{2}{c}{$N_\mathrm{weighted}$} \\\hline
     & \multicolumn{4}{c}{Signal ($m_{\tilde{g}}$ = 1145~\GeV, $m_{\tilde{\chi}_{1}^{\pm}}$ = 785~\GeV, $m_{\tilde{\chi}_{1}^{0}}$ = 425~\GeV)} \\\hline     
No cuts                        & \multicolumn{2}{c}{20000}  &  \multicolumn{2}{c}{ 140.9  } \\
Trigger requirement            & \multicolumn{2}{c}{6788}  &  \multicolumn{2}{c}{  47.6  } \\
Reject events with bad jets    & \multicolumn{2}{c}{6769}  &  \multicolumn{2}{c}{  47.3  } \\
Reject events with bad muons   & \multicolumn{2}{c}{6767}  &  \multicolumn{2}{c}{  47.3  } \\
Primary vertex $\ge 4$ tracks  & \multicolumn{2}{c}{6766}  &  \multicolumn{2}{c}{  47.3  } \\
Veto events with cosmic muons  & \multicolumn{2}{c}{6752}  &  \multicolumn{2}{c}{  47.2  } \\
At least 1 lepton              & \multicolumn{2}{c}{5516}  &  \multicolumn{2}{c}{  38.6  } \\
Fake $E_{\text{T}}^{miss}$     & \multicolumn{2}{c}{5371}  &  \multicolumn{2}{c}{  37.6  } \\
\hline
 & $e$ & $\mu$ & $e$ & $\mu$\\
\hline
Lepton isolation, Trigger matching  & 2116 & 1434 & 14.84 & 10.04  \\\hline
 & \multicolumn{4}{c}{3-jet selection}\\\hline
Jets cut  & 529 & 355 & 14.65  & 9.91 \\ 
\met~cut  & 292 & 177 & 1.91  & 1.29 \\ 
\mt~cut  & 254 & 140 & 1.63   & 1.07  \\ 
\met/\meffincl~cut  & 204 & 113 & 1.59 & 1.03 \\ 
\meffincl~cut  & 203 & 113 & $1.27^{+7.8\%}_{-9.1\%}$ & $0.84^{+16.0\%}_{-11.8\%}$ \\
\hline
$\text{CL}_\text{S}$ obs (exp)   & - & - & 0.66 (0.37) & 0.83 (0.61) \\\hline
%%%%
 & \multicolumn{4}{c}{5-jet selection}\\\hline
Jets cut & 589 & 410 & 11.12  & 7.37 \\ 
\met~cut & 314 & 204 & 5.98  & 3.89 \\ 
\mt~cut & 271& 171 & 4.74 & 2.88 \\
\met/\meffincl~cut & \multicolumn{4}{c}{$-$}\\ 
\meffincl~cut & 271 & 171 & $2.92^{+6.7\%}_{-11.6\%}$ & $1.82^{+6.9\%}_{-6.3\%}$ \\
\hline
$\text{CL}_\text{S}$ obs (exp)  & - & - & 0.42 (0.50) & 0.32 (0.13) \\\hline
%%%%
 & \multicolumn{4}{c}{6-jet selection}\\\hline
Jets cut & 979 & 658  & 7.03  & 4.67  \\ 
\met~cut & 643 & 447  & 2.73  & 2.04  \\ 
\mt~cut & 538 & 364 & 2.38  & 1.69  \\ 
\met/\meffincl~cut &  \multicolumn{4}{c}{$-$}\\ 
\meffincl~cut & 538 & 364 & $2.38^{+9.8\%}_{-10.6\%}$ & $1.69^{+12.0\%}_{-11.8\%}$\\
\hline
$\text{CL}_\text{S}$ obs (exp)  & - & - & 0.33 (0.32) & 0.24 (0.10)\\  
\end{tabular*}
\end{center}
\caption{Cutflow table for the hard single-lepton signal regions, where specific cut values can be seen in table~\ref{tab:hardlepSR}. The signal point is taken from the gluino simplified model with x = 1/2 normalised to 20.3~\ifb; 20000 events were generated for this point. 
The total experimental systematic uncertainty on the signal yield is indicated at the last cut defining each signal region, along with the corresponding observed and expected $\text{CL}_\text{S}$ values.
%The systematic and statistical uncertainties on the signal yield are shown in the signal region. The last row shows the observed and the expected $\text{CL}_\text{S}$ values for the given point. 
\label{table.results.cutflow.SR3Jele}}
\end{table}

\clearpage
\begin{table}
\scriptsize
\begin{center}
\setlength{\tabcolsep}{0.0pc}
\begin{tabular*}{\textwidth}{@{\extracolsep{\fill}}lcccc}
\noalign{\smallskip}\hline\noalign{\smallskip}
Cut     & & & &\\
     & \multicolumn{2}{c}{$N_\mathrm{raw}$} & \multicolumn{2}{c}{$N_\mathrm{weighted}$} \\\hline
 & \multicolumn{4}{c}{Signal ($m_{\tilde{g}}$ = 1025~\GeV, $m_{\tilde{\chi}_{1}^{\pm}}$ = 545~\GeV, $m_{\tilde{\chi}_{1}^{0}}$ = 65~\GeV)} \\\hline
No cuts                        &  \multicolumn{2}{c}{19999}  & \multicolumn{2}{c}{ 396.2  } \\
Trigger requirement            &  \multicolumn{2}{c}{6757}  & \multicolumn{2}{c}{ 132.8  } \\
Reject events with bad jets    & \multicolumn{2}{c}{6731}   & \multicolumn{2}{c}{ 131.6  } \\
Reject events with bad muons   &  \multicolumn{2}{c}{6731}  & \multicolumn{2}{c}{ 131.6  } \\
Primary vertex $\ge 4$ tracks  &  \multicolumn{2}{c}{6730}  & \multicolumn{2}{c}{ 131.6  } \\
Veto events with cosmic muons  & \multicolumn{2}{c}{6715}   & \multicolumn{2}{c}{ 131.3  } \\
At least 1 lepton             &  \multicolumn{2}{c}{5386}   & \multicolumn{2}{c}{ 105.4  } \\
Fake $E_{\text{T}}^{miss}$     &  \multicolumn{2}{c}{5224}  & \multicolumn{2}{c}{ 102.4  } \\
\hline
 & $e$ & $\mu$ & $e$ & $\mu$\\
\hline
Lepton isolation, Trigger matching  & 2040 & 1477& 39.98  & 28.68 \\
\hline
 & \multicolumn{4}{c}{3-jet selection}\\\hline
Jets cut              & 424 & 257 & 39.87  & 28.56 \\ 
\met~cut              & 248 & 145 & 5.63   & 3.92  \\ 
\mt~cut               & 204 & 114 & 4.76   & 3.05 \\
\met/\meffincl~cut    & 130  & 77 & 4.25   & 2.79 \\ 
\meffincl~cut & 130 & 77 & $3.81^{+6.4\%}_{-10.7\%}$ & $2.58^{+12.4\%}_{-10.1\%}$ \\ 
\hline
$\text{CL}_\text{S}$ obs (exp)  & - & - & 0.24 (0.38) & 0.57 (0.69) \\ \hline
 & \multicolumn{4}{c}{5-jet selection}\\\hline
Jets cut               & 545 & 410 &  31.60 & 23.27  \\ 
\met~cut               & 296 & 212 &  16.90 & 12.67  \\ 
\mt~cut                & 250 & 171 &  13.03 & 8.96   \\ 
\met/\meffincl~cut     & \multicolumn{4}{c}{$-$}\\ 
\meffincl~cut  & 250 & 171 & $10.76^{+5.7\%}_{-4.5\%}$ & $7.21^{+5.1\%}_{-5.7\%}$\\ 
\hline
$\text{CL}_\text{S}$ obs (exp)  & - & - & 0.011 (0.50) & 0.008 (0.16) \\ \hline
 & \multicolumn{4}{c}{6-jet selection}\\\hline
Jets cut              & 719 & 808 &  20.99 & 15.82 \\ 
\met~cut              & 719 & 540 &  8.55  & 6.33  \\ 
\mt~cut               & 605 & 418 &  7.34  & 5.09  \\ 
\met/\meffincl~cut    &\multicolumn{4}{c}{$-$}\\ 
\meffincl~cut & 605 & 418 & $7.34^{+5.7\%}_{-8.5\%}$ & $5.09^{+10.6\%}_{-11.9\%}$\\ 
\hline
$\text{CL}_\text{S}$ obs (exp)  & - & - & 0.021 (0.34) & 0.015 (0.13)\\ \hline
\end{tabular*}
\end{center}
\caption{Cutflow table for the hard single-lepton signal regions, where specific cut values can be seen in table~\ref{tab:hardlepSR}. The signal point is taken from the gluino simplified model with x = 1/2 normalised to 20.3~\ifb; 20000 events were generated for this point. 
The total experimental systematic uncertainty on the signal yield is indicated at the last cut defining each signal region, along with the corresponding observed and expected $\text{CL}_\text{S}$ values.
%The systematic and statistical uncertainties on the signal yield are shown in the signal region. The last row shows the observed and the expected $\text{CL}_\text{S}$ values for the given point. 
\label{table.results.cutflow.SR3Jele2}}
\end{table}

\begin{table}
\begin{center}
\footnotesize
\begin{tabular}{lcccccc}
\noalign{\smallskip}\hline\noalign{\smallskip}
%\hline
{\bf cut}                       & \multicolumn{3}{c}{$N_{\text{raw}}$} & \multicolumn{3}{c}{scaled to luminosity}  \\
\hline\hline
No cuts                         & \multicolumn{3}{c}{40000} & \multicolumn{3}{c}{222.9}  \\
Lepton trigger requirement      & \multicolumn{3}{c}{31160} & \multicolumn{3}{c}{173.7}  \\
Reject events with bad jets     & \multicolumn{3}{c}{31000} & \multicolumn{3}{c}{172.8}  \\
Reject events with bad muons    & \multicolumn{3}{c}{30985} & \multicolumn{3}{c}{172.7}  \\
Primary vertex $\ge 4$ tracks   & \multicolumn{3}{c}{30979} & \multicolumn{3}{c}{172.7}  \\
Veto events with cosmic muons   & \multicolumn{3}{c}{30776} & \multicolumn{3}{c}{171.6}  \\
At least 2 leptons              & \multicolumn{3}{c}{14605} & \multicolumn{3}{c}{81.4}  \\
Fake $E_{\text{T}}^{miss}$      & \multicolumn{3}{c}{14569} & \multicolumn{3}{c}{81.2}  \\
$m_{\ell\ell}>20$ GeV           & \multicolumn{3}{c}{14524} & \multicolumn{3}{c}{81.0}  \\
\hline
\multirow{2}{*}{{\bf  channel}}          & \multicolumn{2}{c}{$ee$}  & \multicolumn{2}{c}{$\mu\mu$}   &  \multicolumn{2}{c}{$e\mu$}  \\
& $N_{\text{raw}}$ & $N_{\text{weighted}}$ &$N_{\text{raw}}$ & $N_{\text{weighted}}$  & $N_{\text{raw}}$ & $N_{\text{weighted}}$   \\
%\noalign{\smallskip}\hline\noalign{\smallskip}
\hline\hline
%Trigger + $\ge 2$ preselected & \multicolumn{3}{c}{\multirow{2}{*}{65.13}} \\
%leptons + $m_{\ell\ell}>20$ \GeV           &   & &  \\
%\hline
Lepton flavour                             & 5715 & 25.63   &  4400 & 19.61 & 5269 & 23.63  \\ 
Isolated leptons                           & 4734 & 21.23   &  4097 & 18.28 & 4547 & 20.39  \\ 
Trigger matched leptons                    & 4717 & 21.15   &  3926 & 17.53 & 3745 & 16.79  \\ 
Prompt leptons                             & 4698 & 21.06   &  3926 & 17.53 & 3733 & 16.74  \\ 
$Z$-veto                                   & 4524 & 20.28   &  3759 & 16.85 & \multicolumn{2}{c}{N/A}    \\ 
Poorly reconstructed muons                 & 4523 & 20.28   &  3747 & 16.80 & 3725 & 16.70  \\ 
Electron crack veto                        & 4237 & 19.00   &  3725 & 16.70 & 3450 & 16.11  \\ 
$b$-veto                                   & 3764 & 16.87   &  3374 & 15.13 & 3227 & 14.47  \\ 
\hline
$<3$ jets                                  & 1494 & 6.70    &  1424 & 6.39  & 1495 & 6.70    \\
$R>0.5$                                    & 463  & 2.07    &  426  & 1.91  & 446  & 2.00    \\
$M_{R}'>600$ \GeV   &  411 & $1.84^{+6.7\%}_{-7.1\%}$  & 377 & $1.69^{+6.2\%}_{-7.1\%}$ & 365 & $1.64^{+5.5\%}_{-5.6\%}$  \\ [4pt]
\hline
%$M_{R}'>600$ \GeV   &  $1.84\pm1.36$ $^{+6.7\%}_{-7.1\%}$  & $1.69\pm1.30$ $^{+6.2\%}_{-7.1\%}$ & $1.64\pm1.28$ $^{+5.5\%}_{-5.6\%}$  \\ [4pt]
$\text{CL}_\text{S}$ obs (exp)             &  \multicolumn{2}{c}{0.53 (0.63)}  & \multicolumn{2}{c}{0.68 (0.65)} & \multicolumn{2}{c}{0.63 (0.80)} \\
\hline\hline
$>2$ jets                                  & 2270 & 10.18   & 1855 & 8.74   & 1950 & 8.31    \\
$R>0.35$                                   & 1123 & 5.04    & 988  & 4.43   & 893  & 4.00    \\
$M_{R}'>800$ \GeV   &  841 & $3.77^{+6.4\%}_{-7.0\%}$  & 751 & $3.37^{+7.1\%}_{-5.7\%}$ & 674 & $3.02^{+5.8\%}_{-6.0\%}$ \\ [4pt]
%$M_{R}'>800$ \GeV   &  $3.77\pm1.94$ $^{+6.4\%}_{-7.0\%}$  & $3.37\pm1.83$ $^{+7.1\%}_{-5.7\%}$ & $3.02\pm1.74$ $^{+5.8\%}_{-6.0\%}$ \\ [4pt]
\hline
$\text{CL}_\text{S}$ obs (exp)             &  \multicolumn{2}{c}{0.13 (0.24)} & \multicolumn{2}{c}{0.13 (0.27)} & \multicolumn{2}{c}{0.42 (0.50)} \\
\hline\hline
 \end{tabular}
\end{center}
 \caption{Cutflow table for the hard dilepton channels for an example squark-squark two-step benchmark point (decays via sleptons) with $m_{\tilde{q}}=825$ \GeV, $m_{LSP}=105$ \GeV; 40000 events were generated for this point. Shown here is both the unweighted number of events and the number of events with the sample normalised to 20.3 fb$^{-1}$. The total experimental systematic uncertainty on the signal yield is indicated at the last cut defining each signal region, along with the corresponding observed and expected $\text{CL}_\text{S}$ values.
 \label{tab:cutflow}
 }
\end{table}

\clearpage
\subsubsection{Information on various signal grids}

%\begin{figure}[htb]
%\centering
%\includegraphics[width=0.4\textwidth]{../../INT/SoftLepton/figures/Appendix/ISR_Auxiliary/NGeneventsGG1step_gridx__LSPEE60.eps}
%\includegraphics[width=0.4\textwidth]{../../INT/SoftLepton/figures/Appendix/ISR_Auxiliary/NGeneventsGG1step__LSPNE60.eps}
%\includegraphics[width=0.4\textwidth]{../../INT/SoftLepton/figures/Appendix/ISR_Auxiliary/NGeneventsSS1step_gridx__LSPEE60.eps}
%\includegraphics[width=0.4\textwidth]{../../INT/SoftLepton/figures/Appendix/ISR_Auxiliary/NGeneventsSS1step__LSPNE60.eps}
%\caption{
%Number of generated events in the simplified model of gluino (top) or squark (bottom) pair production decaying in one step with varying x (left) or x=1/2 (right).
%} \label{fig:Ngen}
%\end{figure}
%
%\begin{figure}[htb]
%\centering
%\includegraphics[width=0.4\textwidth]{../../INT/SoftLepton/figures/Appendix/ISR_Auxiliary/XsecGG1step_gridx__LSPEE60.eps}
%\includegraphics[width=0.4\textwidth]{../../INT/SoftLepton/figures/Appendix/ISR_Auxiliary/XsecGG1step__LSPNE60.eps}
%\includegraphics[width=0.4\textwidth]{../../INT/SoftLepton/figures/Appendix/ISR_Auxiliary/XsecSS1step_gridx__LSPEE60.eps}
%\includegraphics[width=0.4\textwidth]{../../INT/SoftLepton/figures/Appendix/ISR_Auxiliary/XsecSS1step__LSPNE60.eps}
%\caption{
%Production cross section in the simplified model of gluino (top) or squark (bottom) pair production decaying in one step with varying x (left) or x=1/2 (right).
%} \label{fig:xSEC}
%\end{figure}

\begin{figure}[htb]
\centering
\includegraphics[width=0.49\textwidth]{figures/nGenEvents_SM_GG_onestepCC.eps}
\includegraphics[width=0.49\textwidth]{figures/SigXSec_SM_GG_onestep.eps}
\caption{
Number of generated events (left) and production cross section (right) in the simplified model of gluino pair production decaying in one step with x=1/2.
} \label{fig:NgenSMGG}
\end{figure}

\begin{figure}[htb]
\centering
\includegraphics[width=0.49\textwidth]{figures/nGenEvents_SM_SS_onestepCCx.eps}
\includegraphics[width=0.49\textwidth]{figures/SigXSec_SM_SS_onestepx.eps}
\caption{
Number of generated events (left) and production cross section (right) in the simplified model of squark pair production decaying in one step with varying x.
} \label{fig:NgenSMSSx}
\end{figure}

\begin{figure}[htb]
\centering
\includegraphics[width=0.49\textwidth]{figures/nGenEvents_MUED.eps}
\includegraphics[width=0.49\textwidth]{figures/SigXSec_MUED.eps}
\caption{
Number of generated events divided by the generator filter efficiency (left) and production cross section (right) in the mUED model.
} \label{fig:Ngen}
\end{figure}

\begin{figure}[htb]
\centering
\includegraphics[width=0.49\textwidth]{figures/nGenEvents_SMSS2CNsl.eps}
\includegraphics[width=0.49\textwidth]{figures/SigXSec_SMSS2CNsl.eps}
\caption{
Number of generated events (left) and production cross section (right) in the simplified model of squark pair production decaying in two steps via sleptons.
} \label{fig:NgenSS2CNsl}
\end{figure}

\clearpage
\subsubsection{Signal region acceptance, efficiency, CLs and systematic uncertainties for representative signal grids}

\begin{figure}[htb]
\centering
\includegraphics[width=0.49\textwidth]{../../INT/SoftLepton/figures/Appendix/ISR_Auxiliary/AccGG1step__LSPNE60_3JE.eps}
\includegraphics[width=0.49\textwidth]{../../INT/SoftLepton/figures/Appendix/ISR_Auxiliary/EffGG1step__LSPNE60_3JE.eps}
\includegraphics[width=0.49\textwidth]{../../INT/SoftLepton/figures/Appendix/ISR_Auxiliary/AccGG1step__LSPNE60_5JE.eps}
\includegraphics[width=0.49\textwidth]{../../INT/SoftLepton/figures/Appendix/ISR_Auxiliary/EffGG1step__LSPNE60_5JE.eps}
\includegraphics[width=0.49\textwidth]{../../INT/SoftLepton/figures/Appendix/ISR_Auxiliary/AccSS1step_gridx__LSPEE60_3JI.eps}
\includegraphics[width=0.49\textwidth]{../../INT/SoftLepton/figures/Appendix/ISR_Auxiliary/EffSS1step_gridx__LSPEE60_3JI.eps}
\caption{
Acceptance (left) and efficiency (right) for the soft single-lepton 3-jet (top), 5-jet (middle) and 3-jet inclusive (bottom) signal regions in
the simplified model of a gluino pair production decaying in one step with x=1/2 (3-jet and 5-jet signal regions) or of a squark pair production decaying in one step with varying x (3-jet inclusive signal region).
} \label{fig:softAxE}
\end{figure}

%jlorenz: want to show plots from combination only
%\begin{figure}[htb]
%\centering
%\includegraphics[width=0.4\textwidth]{../../INT/SoftLepton/figures/Appendix/ISR_Auxiliary/CLsGG1step_gridx__LSPEE60.eps}
%\includegraphics[width=0.4\textwidth]{../../INT/SoftLepton/figures/Appendix/ISR_Auxiliary/CLsGG1step__LSPNE60.eps}
%\includegraphics[width=0.4\textwidth]{../../INT/SoftLepton/figures/Appendix/ISR_Auxiliary/CLsSS1step_gridx__LSPEE60.eps}
%\includegraphics[width=0.4\textwidth]{../../INT/SoftLepton/figures/Appendix/ISR_Auxiliary/CLsSS1step__LSPNE60.eps}
%\caption{
%Observed CLs from the single soft-lepton signal regions in the simplified model of gluino (top) or squark (bottom) pair production decaying in one step with varying x (left) %or x=1/2 (right).
%} \label{fig:softCLs}
%\end{figure}

%\begin{figure}[htb]
%\centering
%\includegraphics[width=0.4\textwidth]{../../INT/SoftLepton/figures/Appendix/ISR_Auxiliary/ExpCLsGG1step_gridx__LSPEE60.eps}
%\includegraphics[width=0.4\textwidth]{../../INT/SoftLepton/figures/Appendix/ISR_Auxiliary/ExpCLsGG1step__LSPNE60.eps}
%\includegraphics[width=0.4\textwidth]{../../INT/SoftLepton/figures/Appendix/ISR_Auxiliary/ExpCLsSS1step_gridx__LSPEE60.eps}
%\includegraphics[width=0.4\textwidth]{../../INT/SoftLepton/figures/Appendix/ISR_Auxiliary/ExpCLsSS1step__LSPNE60.eps}
%\caption{
%Expected CLs from the single soft-lepton signal regions in the simplified model of gluino (top) or squark (bottom) pair production decaying in one step with varying x (left) %or x=1/2 (right).
%} \label{fig:softCLsExp}
%\end{figure}

\begin{figure}[htb]
\centering
\includegraphics[width=0.49\textwidth]{figures/limit_CLsexp_GG1stepx12_combhardsoft_version120115.eps}
\includegraphics[width=0.49\textwidth]{figures/limit_CLsexp_SS1stepgridx_combhardsoft_version170914.eps}
\includegraphics[width=0.49\textwidth]{figures/limit_CLs_GG1stepx12_combhardsoft_version120115.eps}
\includegraphics[width=0.49\textwidth]{figures/limit_CLs_SS1stepgridx_combhardsoft_version170914.eps}
\caption{
Expected (top) and observed (bottom) CLs from the full statistical combination of the single hard-lepton and single soft-lepton signal regions in the simplified model of gluino (left) or squark (right) pair production decaying in one step with x=1/2 (right) or varying x (left).
} \label{fig:combCLs}
\end{figure}

\begin{figure}[htb]
\centering
\includegraphics[width=0.49\textwidth]{figures/AcceptanceUED.eps}
\includegraphics[width=0.49\textwidth]{figures/EfficiencyUED.eps}
\caption{
Acceptance (left) and efficiency (right) for the soft dimuon signal region in the mUED model.
} \label{fig:softdimuAxE}
\end{figure}

\begin{figure}[htb]
\centering
\includegraphics[width=0.49\textwidth]{figures/acc_SMSS2CNslSR_EM_HM.eps}
\includegraphics[width=0.49\textwidth]{figures/eff_SMSS2CNslSR_EM_HM.eps}
\includegraphics[width=0.49\textwidth]{figures/acc_SMSS2CNslSR_SF_HM.eps}
\includegraphics[width=0.49\textwidth]{figures/eff_SMSS2CNslSR_SF_HM.eps}
\includegraphics[width=0.49\textwidth]{figures/acc_SMSS2CNslSR_EM_LM.eps}
\includegraphics[width=0.49\textwidth]{figures/eff_SMSS2CNslSR_EM_LM.eps}
\includegraphics[width=0.49\textwidth]{figures/acc_SMSS2CNslSR_SF_LM.eps}
\includegraphics[width=0.49\textwidth]{figures/eff_SMSS2CNslSR_SF_LM.eps}
\caption{
Acceptance (left) and efficiency (right) for the hard dilepton 3-jet opposite flavour (top row), 3-jet same-flavour (second row),
low-multiplicity opposite-flavour (third row) and low-multiplicity same-flavour (last row) signal regions in the simplified model with squark pair production in which
there is a two-step squark decay through sleptons.
} \label{fig:harddilepAcc}
\end{figure}

\begin{figure}[htb]
\centering
\includegraphics[width=0.49\textwidth]{figures/winner_MUED_.eps}
\caption{
Signal region giving the best expected limit for each point in the mUED model: soft dimuon signal region (D) or hard dilepton signal region (T).
} \label{fig:bestMUED}
\end{figure}

\begin{figure}[htb]
\centering
\includegraphics[width=0.49\textwidth]{figures/CLs_SMSS2CNsl_2_Hard_Lepton_Exp.eps}
\includegraphics[width=0.49\textwidth]{figures/CLs_SMSS2CNsl_2_Hard_Lepton_Obs.eps}
\caption{
Expected (left) and observed (right) CLs in the simplified model of quark pair production decaying in two steps via sleptons.
} \label{fig:CLsSMSS2CNsl}
\end{figure}

	\begin{figure}[htb]
\centering
\includegraphics[width=0.49\textwidth]{figures/CLs_MUED__FullOR_Exp.eps}
\includegraphics[width=0.49\textwidth]{figures/CLs_MUED__FullOR_Obs.eps}
\caption{
Expected (left) and observed (right) CLs in the mUED model.
} \label{fig:CLsMUED}
\end{figure}

\begin{figure}[htb]
\centering
  \includegraphics[width=0.49\textwidth]{figures/accept_SR3JdiscoveryEM_x12.eps}
  \includegraphics[width=0.49\textwidth]{figures/Eff_SR3JdiscoveryEM_x12.eps}\\
  \includegraphics[width=0.49\textwidth]{figures/accept_SR5JdiscoveryEM_x12.eps}
  \includegraphics[width=0.49\textwidth]{figures/Eff_SR5JdiscoveryEM_x12.eps}\\
  \includegraphics[width=0.49\textwidth]{figures/accept_SR6JdiscoveryEM_x12.eps}
  \includegraphics[width=0.49\textwidth]{figures/Eff_SR6JdiscoveryEM_x12.eps}\\
\caption{
Acceptance (left) and efficiency (right) for the hard single-lepton 3-jet (top), 5-jet (middle) and 3-jet (bottom) signal regions in
the simplified model of a gluino pair production decaying in one step with x=1/2.
  } \label{fig.GlGl.AcceptEff}
\end{figure}

\begin{figure}[htb]
\centering
  \includegraphics[width=0.49\textwidth]{figures/accept_SR3JdiscoveryEM_SS1Stepx.eps}
  \includegraphics[width=0.49\textwidth]{figures/Eff_SR3JdiscoveryEM_SS1Stepx.eps}\\
  \includegraphics[width=0.49\textwidth]{figures/accept_SR5JdiscoveryEM_SS1Stepx.eps}
  \includegraphics[width=0.49\textwidth]{figures/Eff_SR5JdiscoveryEM_SS1Stepx.eps}\\
  \includegraphics[width=0.49\textwidth]{figures/accept_SR6JdiscoveryEM_SS1Stepx.eps}
  \includegraphics[width=0.49\textwidth]{figures/Eff_SR6JdiscoveryEM_SS1Stepx.eps}\\
\caption{
Acceptance (left) and efficiency (right) for the hard single-lepton 3-jet (top), 5-jet (middle) and 3-jet (bottom) signal regions in
the simplified model of a squark pair production decaying in one step with varying x.
  } \label{fig.SqSq.AcceptEff}
\end{figure}

\clearpage
\subsubsection{Observed upper limit on the signal cross section for selected signal grids}

\begin{figure}[htb]
\centering
  \includegraphics[width=0.49\textwidth]{figures/limit_contour_GG1stepx12_combhardsoft_version120115_up_EXP.eps}
  \includegraphics[width=0.49\textwidth]{figures/limit_contour_SS1stepgridx_combhardsoft_version141114_up_EXP.eps}
\caption{Expected and observed exclusion limit for the full statistical combination of the single hard-lepton and single soft-lepton signal regions in the simplified model of gluino (left) or squark (right) pair production decaying in one step with x=1/2 (right) or varying x (left).
95 \% C.L. upper limits on the visible cross section are shown.
  } \label{fig:1step_UL}
\end{figure}

\begin{figure}[htb]
\centering
  \includegraphics[width=0.49\textwidth]{../../INT/TwoLepton/figures/Results/Limits/limit_SS_sl_2L_UL.eps}\\
\caption{
        Expected and observed exclusion limits for a simplified model with squark pair production where each squark decays to a quark and chargino, 
        and the chargino subsequently decays through a slepton or sneutrino to the LSP. 95 \% C.L. upper limits on the visible cross section are shown.
  } \label{fig:SMSS2CNsl_UL}
\end{figure}

\begin{figure}[htb]
\centering
  \includegraphics[width=0.49\textwidth]{figures/MUED_combo_UL.eps}\\
\caption{
        Expected and observed exclusion limits from the combination of the soft dimuon and hard dilepton channels in the mUED model, presented in the $1/Rc$--$ΛR_{\mathrm{c}}$ plane. The dark grey dashed line shows the expected limits at 95 \% C.L., with the light (yellow) bands indicating the $\pm 1 \sigma$ variation on the median expected limit due to the experimental and background-only theory uncertainties. 
The observed nominal limit is shown by a solid
dark red line, with the dark red dotted lines indicating the $\pm1\sigma$ variation on this limit due to the theoretical scale and PDF uncertainties on 
the signal cross section. The blue and green full (dashed) lines show the observed (expected) exclusion obtained by the soft dimuon and hard dilepton analyses, respectively. 95 \% C.L. upper limits on the visible cross section are shown.
  } \label{fig:MUED_UL}
\end{figure}

\begin{figure}[htb]
\centering
  \includegraphics[width=0.49\textwidth]{figures/limit_contour_SS2WWZZ_version141114_unblinded_cleaned_up_EXP.eps}
\caption{
Exclusion limits from the hard single-lepton channel in the two-step first- and second-generation squark simplified model without sleptons.
The observed nominal limit is shown by a solid
dark red line, with the dark red dotted lines indicating the $\pm1\sigma$ variation on this limit due to the theoretical scale and PDF uncertainties on 
the signal cross section.
The grey numbers show the upper limit on the production cross section, in pb, obtained for each point of the grids.
There is no expected exclusion limit, as the analysis has no expected sensitivity in this plane.
  } \label{fig:squark_WWZZ}
\end{figure}

\subsubsection{Bin-by-bin yields tables for signal region plots}

\begin{table}
\begin{center}
\setlength{\tabcolsep}{0.0pc}
{\footnotesize
\begin{tabular*}{\textwidth}{@{\extracolsep{\fill}}lrrrrrr}
\noalign{\smallskip}\hline\noalign{\smallskip}
{\bf Figure \ref{fig:SRplots_isr} (top left)}           & total       & bin 1       & bin 2      & bin 3      & bin 4 & bin 5  \\[-0.05cm]
\noalign{\smallskip}\hline\noalign{\smallskip}
Observed events  &     $8$              & $1$              & $0$              & $2$              & $4$   & $1$      \\
\noalign{\smallskip}\hline\noalign{\smallskip}
Fitted bkg events    &  $8.1 \pm 1.6$          & $0.1_{-0.1}^{+0.2}$          & $0.4 \pm 0.2$          & $2.4 \pm 0.9$          & $5.2 \pm 1.1$          & $0.1 \pm 0.1$    \\
\noalign{\smallskip}\hline\noalign{\smallskip}
MC exp.  $m_{\tilde{q}}=425 \GeV, m_{\tilde{\chi}^{\pm}_{1}}=385 \GeV$ &   \multirow{2}{*}{$3.0 \pm 1.2$}  & \multirow{2}{*}{$0.0_{-0.0}^{+0.37}$} & \multirow{2}{*}{$0.0_{-0.0}^{+0.37}$}         & \multirow{2}{*}{$0.5_{-0.5}^{+0.7}$}          & \multirow{2}{*}{$2.5 \pm 1.6$}   & \multirow{2}{*}{$0.0_{-0.0}^{+0.37}$}      \\
and $m_{\tilde{\chi}^0_1}=345 \GeV$ events         & &&&&         \\
\noalign{\smallskip}\hline\noalign{\smallskip}
\end{tabular*}
%%%
}
\end{center}
\caption{
Table shows the data, fitted background and expected signal event counts for a benchmark signal point in each bin of the \MET/\meff~distribution shown in figure~\ref{fig:SRplots_isr} (top left). 
The fit results are shown for an integrated luminosity of $20.1$ \ifb. 
Combined systematic and statistical uncertainties are indicated. 
}
\label{tab:softSR1L3j_bins}
\end{table}

\begin{table}
\begin{center}
\setlength{\tabcolsep}{0.0pc}
{\footnotesize
\begin{tabular*}{\textwidth}{@{\extracolsep{\fill}}lrrrrrr}
\noalign{\smallskip}\hline\noalign{\smallskip}
{\bf Figure \ref{fig:SRplots_isr} (top right)}           & total       & bin 1       & bin 2      & bin 3      & bin 4 & bin 5   \\[-0.05cm]
\noalign{\smallskip}\hline\noalign{\smallskip}
Observed events  & $19$              & $0$              & $8$              & $7$              & $4$  & $0$   \\
\noalign{\smallskip}\hline\noalign{\smallskip}
Fitted bkg events    & $27.7 \pm 7.0$          & $1.0 \pm 0.6$          & $10.8 \pm 3.1$          & $12.4 \pm 3.0$          & $3.5 \pm 1.0$          & $0.0_{-0.0}^{+1.14}$ \\
\noalign{\smallskip}\hline\noalign{\smallskip}
MC exp.  $m_{\tilde{g}}=625 \GeV, m_{\tilde{\chi}^{\pm}_{1}}=545 \GeV$ &    \multirow{2}{*}{$22.2 \pm 10.8$}          & \multirow{2}{*}{$0.0_{-0.0}^{+1.13}$}         & \multirow{2}{*}{$3.0_{-3.0}^{+3.4}$}         & \multirow{2}{*}{$11.0 \pm 5.9$}          & \multirow{2}{*}{$8.2 \pm 3.7$}  & \multirow{2}{*}{$0.0_{-0.0}^{+1.13}$}     \\
and $m_{\tilde{\chi}^0_1}=465 \GeV$ events         & &&&&         \\
\noalign{\smallskip}\hline\noalign{\smallskip}
\end{tabular*}
%%%
}
\end{center}
\caption{
Table shows the data, fitted background and expected signal event counts for a benchmark signal point in each bin of the \MET/\meff~distribution shown in figure~\ref{fig:SRplots_isr} (top right). 
The fit results are shown for an integrated luminosity of $20.1$ \ifb. 
Combined systematic and statistical uncertainties are indicated. 
}
\label{tab:softSR1L5j_bins}
\end{table}

\begin{table}
\begin{center}
\setlength{\tabcolsep}{0.0pc}
{\footnotesize
\begin{tabular*}{\textwidth}{@{\extracolsep{\fill}}lrrrrrr}
\noalign{\smallskip}\hline\noalign{\smallskip}
{\bf Figure \ref{fig:SRplots_isr} (bottom left)}           & total       & bin 1       & bin 2      & bin 3      & bin 4  & bin 5 \\[-0.05cm]
\noalign{\smallskip}\hline\noalign{\smallskip}
Observed events  &  $34$              & $2$              & $11$              & $14$              & $7$     & $0$             \\
\noalign{\smallskip}\hline\noalign{\smallskip}
Fitted bkg events    &     $37.0 \pm 6.7$          & $1.6 \pm 1.0$          & $14.3 \pm 3.5$          & $13.3 \pm 2.6$          & $7.6 \pm 1.3$          & $0.2 \pm 0.1$                       \\
\noalign{\smallskip}\hline\noalign{\smallskip}
MC exp.  $m_{\tilde{q}}=300 \GeV, m_{\tilde{\chi}^{\pm}_{1}}=110 \GeV$ &   \multirow{2}{*}{$40.2 \pm 17.4$}         & \multirow{2}{*}{$4.5 \pm 3.1$}          & \multirow{2}{*}{$12.9 \pm 9.8$}          & \multirow{2}{*}{$13.4 \pm 8.9$}         & \multirow{2}{*}{$9.4 \pm 7.2$}      & \multirow{2}{*}{$0.0_{-0.0}^{+3.03}$}           \\
and $m_{\tilde{\chi}^0_1}=60 \GeV$ events         & &&&&         \\
\noalign{\smallskip}\hline\noalign{\smallskip}
\end{tabular*}
%%%
}
\end{center}
\caption{
Table shows the data, fitted background and expected signal event counts for a benchmark signal point in each bin of the \MET/\meff~distribution shown in figure~\ref{fig:SRplots_isr} (bottom left). 
The fit results are shown for an integrated luminosity of $20.1$ \ifb. 
Combined systematic and statistical uncertainties are indicated. 
}
\label{tab:softSR1L3jincl_bins}
\end{table}

\begin{table}
\begin{center}
\setlength{\tabcolsep}{0.0pc}
{\footnotesize
\begin{tabular*}{\textwidth}{@{\extracolsep{\fill}}lrrrrr}
\noalign{\smallskip}\hline\noalign{\smallskip}
{\bf Figure \ref{fig:SRplots_isr} (bottom right)}           & total       & bin 1       & bin 2      & bin 3      & bin 4   \\[-0.05cm]
\noalign{\smallskip}\hline\noalign{\smallskip}
Observed events          & 6 & 2 & 2 & 0 & 2 \\
\noalign{\smallskip}\hline\noalign{\smallskip}
Fitted bkg events          & $6.2 \pm 2.9$          & $2.3 \pm 1.2$          & $2.0 \pm 1.0$          & $0.3_{-0.3}^{+0.4}$          & $1.6 \pm 0.8$ \\
%$6.16 \pm 2.88$
\noalign{\smallskip}\hline\noalign{\smallskip}
MC exp.  mUED($R^{-1}_c=1000$ GeV, $\Lambda R_{\mathrm{c}}=5$) events      & $6.28$     & $1.15$          & $0.60$          & $0.55$          & $3.98$              \\
\noalign{\smallskip}\hline\noalign{\smallskip}
\end{tabular*}
%%%
}
\end{center}
\caption{
Table shows the data, fitted background and expected signal event counts for a benchmark signal point in each bin of the \met~distribution shown in figure~\ref{fig:SRplots_isr} (bottom right). 
The fit results are shown for an integrated luminosity of $20.1$ \ifb. 
Combined systematic and statistical uncertainties are indicated. 
}
\label{tab:SR2mu_bins}
\end{table}

\begin{table}
\begin{center}
\setlength{\tabcolsep}{0.0pc}
{\footnotesize
\begin{tabular*}{\textwidth}{@{\extracolsep{\fill}}lrrrrr}
\noalign{\smallskip}\hline\noalign{\smallskip}
{\bf Figure \ref{fig:SRexclAfterFit} (top left)}           & total       & bin 1       & bin 2      & bin 3      & bin 4   \\[-0.05cm]
\noalign{\smallskip}\hline\noalign{\smallskip}
Observed events  & $75$              & $38$              & $21$              & $7$              & $9$                    \\
\noalign{\smallskip}\hline\noalign{\smallskip}
Fitted bkg events    & $82.5 \pm 7.2$          & $39.3 \pm 3.9$          & $26.2 \pm 2.8$          & $8.5 \pm 1.1$          & $8.7 \pm 1.4$  \\
\noalign{\smallskip}\hline\noalign{\smallskip}
MC exp.  $m_{\tilde{g}}=1025 \GeV, m_{\tilde{\chi}^{\pm}_{1}}=545 \GeV$ & \multirow{2}{*}{$4.5 \pm 1.3$}          & \multirow{2}{*}{$0.21 \pm 0.07$}          & \multirow{2}{*}{$1.0 \pm 0.4$}          & \multirow{2}{*}{$1.3 \pm 0.4$}          & \multirow{2}{*}{$2.0 \pm 0.6$}           \\
and $m_{\tilde{\chi}^0_1}=65 \GeV$ events         & &&&&         \\
\noalign{\smallskip}\hline\noalign{\smallskip}
\end{tabular*}
%%%
}
\end{center}
\caption{
Table shows the data, fitted background and expected signal event counts for a benchmark signal point in each bin of the \meffincl~distribution shown in figure~\ref{fig:SRexclAfterFit} (top left). 
The fit results are shown for an integrated luminosity of $20.3$ \ifb. 
Combined systematic and statistical uncertainties are indicated. 
}
\label{tab:SR3JEM_bins}
\end{table}

\begin{table}
\begin{center}
\setlength{\tabcolsep}{0.0pc}
{\footnotesize
\begin{tabular*}{\textwidth}{@{\extracolsep{\fill}}lrrrrr}
\noalign{\smallskip}\hline\noalign{\smallskip}
{\bf Figure \ref{fig:SRexclAfterFit} (top right)}           & total       & bin 1       & bin 2      & bin 3      & bin 4   \\[-0.05cm]
\noalign{\smallskip}\hline\noalign{\smallskip}
Observed events  & $16$              & $7$              & $0$              & $4$              & $5$ \\
\noalign{\smallskip}\hline\noalign{\smallskip}
Fitted bkg events    & $17.7 \pm 4.0$          & $3.0 \pm 0.7$          & $4.5 \pm 1.3$          & $3.80 \pm 0.95$          & $6.4 \pm 1.6$ \\
\noalign{\smallskip}\hline\noalign{\smallskip}
MC exp.  $m_{\tilde{g}}=1025 \GeV, m_{\tilde{\chi}^{\pm}_{1}}=545 \GeV$        &      \multirow{2}{*}{$8.2 \pm 2.3$}          & \multirow{2}{*}{$0.00_{-0.00}^{+0.02}$}          & \multirow{2}{*}{$0.60 \pm 0.21$}          & \multirow{2}{*}{$2.2 \pm 0.6$}          & \multirow{2}{*}{$5.4 \pm 1.5$}      \\
 and $m_{\tilde{\chi}^0_1}=65 \GeV$ events & &&&&\\
\noalign{\smallskip}\hline\noalign{\smallskip}
\end{tabular*}
%%%
}
\end{center}
\caption{
Table shows the data, fitted background and expected signal event counts for a benchmark signal point in each bin of the \meffincl~distribution shown in figure~\ref{fig:SRexclAfterFit} (top right). 
The fit results are shown for an integrated luminosity of $20.3$ \ifb. 
Combined systematic and statistical uncertainties are indicated. 
}
\label{tab:SR5JEM_bins}
\end{table}

\begin{table}
\begin{center}
\setlength{\tabcolsep}{0.0pc}
{\footnotesize
\begin{tabular*}{\textwidth}{@{\extracolsep{\fill}}lrrrr}
\noalign{\smallskip}\hline\noalign{\smallskip}
{\bf Figure \ref{fig:SRexclAfterFit} (bottom)}           & total       & bin 1       & bin 2      & bin 3        \\[-0.05cm]
\noalign{\smallskip}\hline\noalign{\smallskip}
Observed events  & $12$              & $10$              & $2$              & $0$  \\
\noalign{\smallskip}\hline\noalign{\smallskip}
Fitted bkg events    & $18.1 \pm 4.3$          & $13.3 \pm 3.4$          & $3.3 \pm 0.8$          & $1.6 \pm 0.4$   \\
\noalign{\smallskip}\hline\noalign{\smallskip}
MC exp.  $m_{\tilde{g}}=1025 \GeV, m_{\tilde{\chi}^{\pm}_{1}}=545 \GeV$        &  \multirow{2}{*}{$20.4 \pm 5.7$}          & \multirow{2}{*}{$7.9 \pm 2.2$}          & \multirow{2}{*}{$6.2 \pm 1.8$}          & \multirow{2}{*}{$6.3 \pm 1.8$}       \\
 and $m_{\tilde{\chi}^0_1}=65 \GeV$ events & &&& \\
\noalign{\smallskip}\hline\noalign{\smallskip}
\end{tabular*}
%%%
}
\end{center}
\caption{
Table shows the data, fitted background and expected signal event counts for a benchmark signal point in each bin of the \met~distribution shown in figure~\ref{fig:SRexclAfterFit} (bottom). 
The fit results are shown for an integrated luminosity of $20.3$ \ifb. 
Combined systematic and statistical uncertainties are indicated. 
}
\label{tab:SR6JEM_bins}
\end{table}

\input{texfiles/VSR_SF_LM.tex}
\input{texfiles/VSR_SF_HM.tex}
\input{texfiles/VSR_EM_LM.tex}
\input{texfiles/VSR_EM_HM.tex}
